# Supplementary material for: Test-based Patch Clustering for Automatically-Generated Patches Assessment
Source: arXiv:2207.11082 source file (2024-08-27)
Supplement: Supplementary file 1 [file additionalref.tex]

% Encoding: UTF-8

@inproceedings{ssbse18-keynote,
author = "Nadia Alshahwan and Xinbo Gao and Mark Harman and Yue Jia and Ke Mao and Alexander Mols and Taijin Tei and Ilya Zorin",
title = "Deploying Search Based Software Engineering with {S}apienz at {F}acebook (keynote paper)",
booktitle = "$10^{th}$ International Symposium  on Search Based Software Engineering",
  pages     = {3--45},
  year      = {2018}
}
@article{eckhardt1991experimental,
	title={An experimental evaluation of software redundancy as a strategy for improving reliability},
	author={Eckhardt, Dave E and Caglayan, Alper K. and Knight, John C. and Lee, Larry D. and McAllister, David F. and Vouk, Mladen A. and Kelly, John P. J.},
	journal={IEEE Transactions on software engineering},
	volume={17},
	number={7},
	pages={692--702},
	year={1991},
	publisher={IEEE}
}
@inproceedings{prabhu2014fastxml,
  title={Fastxml: A fast, accurate and stable tree-classifier for extreme multi-label learning},
  author={Prabhu, Yashoteja and Varma, Manik},
  booktitle={Proceedings of the 20th ACM SIGKDD international conference on Knowledge discovery and data mining},
  pages={263--272},
  year={2014}
}
@article{madjarov2012extensive,
  title={An extensive experimental comparison of methods for multi-label learning},
  author={Madjarov, Gjorgji and Kocev, Dragi and Gjorgjevikj, Dejan and D{\v{z}}eroski, Sa{\v{s}}o},
  journal={Pattern recognition},
  volume={45},
  number={9},
  pages={3084--3104},
  year={2012},
  publisher={Elsevier}
}
@article{quinlan1996learning,
  title={Learning decision tree classifiers},
  author={Quinlan, J. Ross},
  journal={ACM Computing Surveys (CSUR)},
  volume={28},
  number={1},
  pages={71--72},
  year={1996},
  publisher={ACM New York, NY, USA}
}
@article{ruck1990multilayer,
  title={The multilayer perceptron as an approximation to a Bayes optimal discriminant function},
  author={Ruck, Dennis W and Rogers, Steven K and Kabrisky, Matthew and Oxley, Mark E and Suter, Bruce W},
  journal={IEEE transactions on neural networks},
  volume={1},
  number={4},
  pages={296--298},
  year={1990},
  publisher={IEEE}
}
@article{charte2015mlsmote,
  title={MLSMOTE: approaching imbalanced multilabel learning through synthetic instance generation},
  author={Charte, Francisco and Rivera, Antonio J and del Jesus, Mar{\'\i}a J and Herrera, Francisco},
  journal={Knowledge-Based Systems},
  volume={89},
  pages={385--397},
  year={2015},
  publisher={Elsevier}
}
@inproceedings{smith2012measuring,
  title={Measuring algorithm footprints in instance space},
  author={Smith-Miles, Kate and Tan, Thomas T},
  booktitle={2012 IEEE Congress on Evolutionary Computation},
  pages={1--8},
  year={2012},
  organization={IEEE}
}
@article{Chidamber94,
 author = 	 {Chidamber, S.R. and Kemerer, C.F.},
 title = 	 {A Metrics Suite for Object Oriented Design},
 journal = 	 {IEEE Transactions on Software Engineering},
 year = 	 1994,
 volume =	 20,
 number =	 6,
 pages =	 {476-493}
}
@article{chen2010adaptive,
	title={Adaptive random testing: The art of test case diversity},
	author={Chen, Tsong Yueh and Kuo, Fei-Ching and Merkel, Robert G and Tse, TH},
	journal={Journal of Systems and Software},
	volume={83},
	number={1},
	pages={60--66},
	year={2010},
	publisher={Elsevier}
}
@article{Harman2012,
 author = {Harman, Mark and Mansouri, S. Afshin and Zhang, Yuanyuan},
 title = {Search-based Software Engineering: Trends, Techniques and Applications},
 journal = {ACM Computing Surveys},
 volume = {45},
 number = {1},
 year = {2012},
 issn = {0360-0300},
 pages = {11:1--11:61},
 articleno = {11},
 publisher = {ACM},
} 

%OLD
@article{hall2009weka,
  title={The WEKA data mining software: an update},
  author={Hall, Mark and Frank, Eibe and Holmes, Geoffrey and Pfahringer, Bernhard and Reutemann, Peter and Witten, Ian H},
  journal={ACM SIGKDD explorations newsletter},
  volume={11},
  number={1},
  pages={10--18},
  year={2009},
  publisher={ACM}
}
@inproceedings{shamshiri2015random,
  title={Random or Genetic Algorithm Search for Object-Oriented Test Suite Generation?},
  author={Shamshiri, Sina and Rojas, Jos{\'e} Miguel and Fraser, Gordon and McMinn, Phil},
  booktitle={Proceedings of the 2015 Annual Conference on Genetic and Evolutionary Computation},
  pages={1367--1374},
  year={2015},
  organization={ACM}
}
@inproceedings{arcuri2010formal,
  title={Formal analysis of the effectiveness and predictability of random testing},
  author={Arcuri, Andrea and Iqbal, Muhammad Zohaib and Briand, Lionel},
  booktitle={Proceedings of the 19th international symposium on Software testing and analysis},
  pages={219--230},
  year={2010},
  organization={ACM}
}
@article{panichella:2017b,
	Author = {A. Panichella and F. Kifetew and P. Tonella},
	Date-Added = {2017-11-14 04:30:42 +0000},
	Date-Modified = {2017-11-14 04:31:08 +0000},
	Doi = {10.1109/TSE.2017.2663435},
	Issn = {0098-5589},
	Journal = {IEEE Transactions on Software Engineering},
	Number = {99},
	Pages = {1-1},
	Title = {Automated Test Case Generation as a Many-Objective Optimisation Problem with Dynamic Selection of the Targets},
	Volume = {PP},
	Year = {2017},
	Bdsk-Url-1 = {http://dx.doi.org/10.1109/TSE.2017.2663435}}

@inproceedings{allen:1970,
	Acmid = {808479},
	Address = {New York, NY, USA},
	Author = {Allen, Frances E.},
	Booktitle = {Proceedings of a Symposium on Compiler Optimization},
	Date-Added = {2017-11-14 02:21:45 +0000},
	Date-Modified = {2017-11-14 02:22:28 +0000},
	Doi = {10.1145/800028.808479},
	Location = {Urbana-Champaign, Illinois},
	Numpages = {19},
	Pages = {1--19},
	Publisher = {ACM},
	Title = {Control Flow Analysis},
	Url = {http://doi.acm.org/10.1145/800028.808479},
	Year = {1970},
	Bdsk-Url-1 = {http://doi.acm.org/10.1145/800028.808479},
	Bdsk-Url-2 = {http://dx.doi.org/10.1145/800028.808479}}

@inproceedings{panichella:2015,
	Author = {A. Panichella and F. M. Kifetew and P. Tonella},
	Booktitle = {IEEE International Conference on Software Testing, Verification and Validation},
	Doi = {10.1109/ICST.2015.7102604},
	Issn = {2159-4848},
	Pages = {1-10},
	Title = {Reformulating Branch Coverage as a Many-Objective Optimization Problem},
	Year = {2015},
	Bdsk-Url-1 = {http://dx.doi.org/10.1109/ICST.2015.7102604}}

@article{powers:2013,
	Author = {Powers, D. M. W.},
	Citeulike-Article-Id = {12882259},
	Date-Added = {2017-11-10 13:42:14 +0000},
	Date-Modified = {2017-11-10 13:42:35 +0000},
	Journal = {Journal of Machine Learning Technologies},
	Keywords = {evaluation, metrics, nlp},
	Number = {1},
	Pages = {37--63},
	Posted-At = {2013-12-26 21:07:18},
	Priority = {2},
	Title = {{Evaluation: From precision, recall and f-measure to roc., informedness, markedness \& correlation}},
	Volume = {2},
	Year = {2011}}

@article{rojas:2017,
	Author = {Rojas, Jos{\'e} Miguel and Vivanti, Mattia and Arcuri, Andrea and Fraser, Gordon},
	Doi = {10.1007/s10664-015-9424-2},
	Issn = {1573-7616},
	Journal = {Empirical Software Engineering},
	Number = {2},
	Pages = {852--893},
	Title = {A detailed investigation of the effectiveness of whole test suite generation},
	Volume = {22},
	Year = {2017}
    }

@article{afzal2009systematic,
	Author = {Afzal, Wasif and Torkar, Richard and Feldt, Robert},
	Journal = {Information and Software Technology},
	Number = {6},
	Pages = {957--976},
	Publisher = {Elsevier},
	Title = {A systematic review of search-based testing for non-functional system properties},
	Volume = {51},
	Year = {2009}}
@article{aleti2013software,
  title={Software architecture optimization methods: A systematic literature review},
  author={Aleti, Aldeida and Buhnova, Barbora and Grunske, Lars and Koziolek, Anne and Meedeniya, Indika},
  journal={IEEE Transactions on Software Engineering},
  volume={39},
  number={5},
  pages={658--683},
  year={2013},
  publisher={IEEE}
}
@article{Aleti2015G,
	Author = {Aldeida Aleti and Lars Grunske},
	Doi = {https://doi.org/10.1016/j.jss.2014.11.035},
	Issn = {0164-1212},
	Journal = {Journal of Systems and Software},
	Pages = {343 - 352},
	Title = {Test data generation with a Kalman filter-based adaptive genetic algorithm},
	Volume = {103},
	Year = {2015},
	Bdsk-Url-1 = {https://doi.org/10.1016/j.jss.2014.11.035}}

@article{Aleti2016,
	Author = {Aleti, Aldeida and Moser, I. and Grunske, Lars},
	Doi = {10.1007/s10515-016-0197-7},
	Issn = {1573-7535},
	Journal = {Automated Software Engineering},
	Pages = {1--19},
	Title = {Analysing the fitness landscape of search-based software testing problems},
	Year = {2016},
	Bdsk-Url-1 = {http://dx.doi.org/10.1007/s10515-016-0197-7}}
@ARTICLE{OlivieraAleti, 
author={C. Oliveira and A. Aleti and L. Grunske and K. Smith-Miles}, 
journal={IEEE Transactions on Reliability}, 
title={Mapping the Effectiveness of Automated Test Suite Generation Techniques}, 
year={2018}, 
volume={67}, 
number={3}, 
pages={771-785}, 
doi={10.1109/TR.2018.2832072},}
@article{ali2010systematic,
	Author = {Ali, Shaukat and Briand, Lionel C and Hemmati, Hadi and Panesar-Walawege, Rajwinder Kaur},
	Journal = {IEEE Transactions on Software Engineering},
	Number = {6},
	Pages = {742--762},
	Publisher = {IEEE},
	Title = {A systematic review of the application and empirical investigation of search-based test case generation},
	Volume = {36},
	Year = {2010}}

@inproceedings{alshahwan2011automated,
	Author = {Alshahwan, Nadia and Harman, Mark},
	Booktitle = {Proceedings of the 2011 26th IEEE/ACM International Conference on Automated Software Engineering},
	Organization = {IEEE Computer Society},
	Pages = {3--12},
	Title = {Automated web application testing using search based software engineering},
	Year = {2011}}

@article{anand:2013,
	Author = {Anand, Saswat and Burke, Edmund K. and Chen, Tsong Yueh and Clark, John and Cohen, Myra B. and Grieskamp, Wolfgang and Harman, Mark and Harrold, Mary Jean and Mcminn, Phil},
	Doi = {10.1016/j.jss.2013.02.061},
	Journal = {Journal of Systems Software},
	Number = {8},
	Pages = {1978--2001},
	Title = {An Orchestrated Survey of Methodologies for Automated Software Test Case Generation},
	Volume = {86},
	Year = {2013},}

@article{anderson1985eigenvalues,
	Author = {Anderson Jr, William N and Morley, Thomas D},
	Journal = {Linear and multilinear algebra},
	Number = {2},
	Pages = {141--145},
	Publisher = {Taylor \& Francis},
	Title = {Eigenvalues of the Laplacian of a graph∗},
	Volume = {18},
	Year = {1985}}

@article{arcuri:2014,
	Author = {Arcuri, Andrea and Briand, Lionel},
	Date-Added = {2017-02-20 09:59:06 +0000},
	Date-Modified = {2017-02-20 09:59:19 +0000},
	Journal = {Software Testing, Verification and Reliability},
	Number = {3},
	Pages = {219--250},
	Publisher = {Wiley Online Library},
	Title = {A hitchhiker's guide to statistical tests for assessing randomized algorithms in software engineering},
	Volume = {24},
	Year = {2014}}

@inproceedings{Arcuri:2011,
	Acmid = {2001452},
	Author = {Arcuri, Andrea and Briand, Lionel},
	Booktitle = {Proceedings of the 2011 International Symposium on Software Testing and Analysis},
	Doi = {10.1145/2001420.2001452},
	Isbn = {978-1-4503-0562-4},
	Location = {Toronto, Ontario, Canada},
	Numpages = {11},
	Pages = {265--275},
	Publisher = {ACM},
	Series = {ISSTA '11},
	Title = {Adaptive Random Testing: An Illusion of Effectiveness?},
	Url = {http://doi.acm.org/10.1145/2001420.2001452},
	Year = {2011},
	Bdsk-Url-1 = {http://doi.acm.org/10.1145/2001420.2001452},
	Bdsk-Url-2 = {http://dx.doi.org/10.1145/2001420.2001452}}

@incollection{bauersfeld:2013,
	Author = {Bauersfeld, Sebastian and Vos, Tanja EJ and Lakhotia, Kiran},
	Booktitle = {Future Internet Testing},
	Date-Added = {2016-04-28 05:37:54 +0000},
	Date-Modified = {2016-04-28 05:39:20 +0000},
	Pages = {75--94},
	Publisher = {Springer},
	Title = {Unit Testing Tool Competitions--Lessons Learned},
	Year = {2013}}

@article{birant2007st,
	Author = {Birant, Derya and Kut, Alp},
	Journal = {Data \& Knowledge Engineering},
	Number = {1},
	Pages = {208--221},
	Publisher = {Elsevier},
	Title = {ST-DBSCAN: An algorithm for clustering spatial--temporal data},
	Volume = {60},
	Year = {2007}}

@inproceedings{borah2004improved,
	Author = {Borah, B and Bhattacharyya, DK},
	Booktitle = {Intelligent Sensing and Information Processing, 2004. Proceedings of International Conference on},
	Organization = {IEEE},
	Pages = {92--96},
	Title = {An improved sampling-based DBSCAN for large spatial databases},
	Year = {2004}}

@inproceedings{briand2002using,
	Author = {Briand, Lionel C and Feng, Jie and Labiche, Yvan},
	Booktitle = {Proceedings of the 14th international conference on Software engineering and knowledge engineering},
	Organization = {ACM},
	Pages = {43--50},
	Title = {Using genetic algorithms and coupling measures to devise optimal integration test orders},
	Year = {2002}}

@article{chen2009adaptive,
	Author = {Chen, Tsong Yueh and Kuo, Fei-Ching and Liu, Huai},
	Journal = {Journal of Systems and Software},
	Number = {9},
	Pages = {1419--1433},
	Publisher = {Elsevier},
	Title = {Adaptive random testing based on distribution metrics},
	Volume = {82},
	Year = {2009}}

@inproceedings{chen:2005,
	Author = {Tsong Yueh Chen and Hing Leung and I. K. Mak},
	Booktitle = {Advances in Computer Science - {ASIAN} 2004, Higher-Level Decision Making, 9th Asian Computing Science Conference},
	Pages = {320--329},
	Publisher = {Springer},
	Series = {Lecture Notes in Computer Science},
	Title = {Adaptive Random Testing},
	Volume = {3321},
	Year = {2004}}

@article{chidamber:1994,
	Author = {Chidamber, Shyam R and Kemerer, Chris F},
	Date-Added = {2016-03-16 09:47:26 +0000},
	Date-Modified = {2016-03-16 09:47:39 +0000},
	Journal = {Software Engineering, IEEE Transactions on},
	Number = {6},
	Pages = {476--493},
	Publisher = {IEEE},
	Title = {A metrics suite for object oriented design},
	Volume = {20},
	Year = {1994}}

@phdthesis{chitirala:2015,
	Author = {Chitirala, Sai Charan Raj},
	Date-Added = {2016-03-23 02:48:11 +0000},
	Date-Modified = {2016-03-23 02:48:25 +0000},
	School = {UNIVERSITY OF MINNESOTA},
	Title = {Comparing the effectiveness of automated test generation tools ``EVOSUITE'' and ``Tpalus''},
	Year = {2015}}

@inproceedings{ciupa:2008a,
	Acmid = {1368099},
	Address = {New York, NY, USA},
	Author = {Ciupa, Ilinca and Leitner, Andreas and Oriol, Manuel and Meyer, Bertrand},
	Booktitle = {Proceedings of the 30th International Conference on Software Engineering},
	Date-Added = {2017-02-12 07:29:33 +0000},
	Date-Modified = {2017-02-12 07:29:44 +0000},
	Doi = {10.1145/1368088.1368099},
	Isbn = {978-1-60558-079-1},
	Keywords = {adaptive random testing, object distance, software testing},
	Location = {Leipzig, Germany},
	Numpages = {10},
	Pages = {71--80},
	Publisher = {ACM},
	Series = {ICSE '08},
	Title = {ARTOO: Adaptive Random Testing for Object-oriented Software},
	Url = {http://doi.acm.org/10.1145/1368088.1368099},
	Year = {2008},
	Bdsk-Url-1 = {http://doi.acm.org/10.1145/1368088.1368099},
	Bdsk-Url-2 = {http://dx.doi.org/10.1145/1368088.1368099}}

@inproceedings{ciupa:2008b,
	Author = {Ciupa, Ilinca and Pretschner, Alexander and Leitner, Andreas and Oriol, Manuel and Meyer, Bertrand},
	Booktitle = {Software Testing, Verification, and Validation, 2008 1st International Conference on},
	Date-Added = {2017-02-12 07:31:20 +0000},
	Date-Modified = {2017-02-12 07:31:28 +0000},
	Organization = {IEEE},
	Pages = {72--81},
	Title = {On the predictability of random tests for object-oriented software},
	Year = {2008}}

@inproceedings{colanzi2011integration,
	Author = {Colanzi, Thelma Elita and Assun{\c{c}}{\~a}o, Wesley Klewerton Guez and Vergilio, Silvia Regina and Pozo, Aurora},
	Booktitle = {International Symposium on Search Based Software Engineering},
	Organization = {Springer},
	Pages = {188--203},
	Title = {Integration test of classes and aspects with a multi-evolutionary and coupling-based approach},
	Year = {2011}}

@article{csallner:2004,
	Author = {Csallner, Christoph and Smaragdakis, Yannis},
	Date-Added = {2017-02-15 10:02:52 +0000},
	Date-Modified = {2017-02-15 10:03:09 +0000},
	Doi = {10.1002/spe.602},
	Issn = {1097-024X},
	Journal = {Software: Practice and Experience},
	Keywords = {software testing, test case generation, random testing, Java, state re-initialization},
	Number = {11},
	Pages = {1025--1050},
	Publisher = {John Wiley \& Sons, Ltd.},
	Title = {JCrasher: an automatic robustness tester for Java},
	Url = {http://dx.doi.org/10.1002/spe.602},
	Volume = {34},
	Year = {2004},
	Bdsk-Url-1 = {http://dx.doi.org/10.1002/spe.602}}

@inproceedings{cseppento:2015,
	Author = {Lajos Cseppento and Zolt{\'{a}}n Micskei},
	Bibsource = {dblp computer science bibliography, http://dblp.org},
	Biburl = {http://dblp.uni-trier.de/rec/bib/conf/icst/CseppentoM15},
	Booktitle = {8th {IEEE} International Conference on Software Testing, Verification and Validation, {ICST} 2015, Graz, Austria, April 13-17, 2015},
	Doi = {10.1109/ICST.2015.7102587},
	Pages = {1--10},
	Publisher = {{IEEE} Computer Society},
	Timestamp = {Fri, 05 Aug 2016 12:49:20 +0200},
	Title = {Evaluating Symbolic Execution-Based Test Tools},
	Url = {http://dx.doi.org/10.1109/ICST.2015.7102587},
	Year = {2015},
	Bdsk-Url-1 = {http://dx.doi.org/10.1109/ICST.2015.7102587}}

@inproceedings{daniel2008predicting,
	Author = {Daniel, Brett and Boshernitsan, Marat},
	Booktitle = {Proceedings of the 2008 23rd IEEE/ACM International Conference on Automated Software Engineering},
	Organization = {IEEE Computer Society},
	Pages = {363--366},
	Title = {Predicting effectiveness of automatic testing tools},
	Year = {2008}}

@article{dautovic:2011,
	Author = {Dautovic, Andreas and Gonzalez-Sanchez, Alberto and Abreu, Rui and Gross, Hans-Gerhard and van Gemund, Arjan JC},
	Date-Added = {2017-02-12 12:38:49 +0000},
	Date-Modified = {2017-02-12 12:38:58 +0000},
	Title = {2011 26th IEEE/ACM International Conference on Automated Software Engineering (ASE)}}

@inproceedings{dave2015search,
	Author = {Dave, Meenu and Agrawal, Rashmi},
	Booktitle = {Advance Computing Conference (IACC), 2015 IEEE International},
	Organization = {IEEE},
	Pages = {795--799},
	Title = {Search based techniques and mutation analysis in automatic test case generation: a survey},
	Year = {2015}}
@book{kaner2008lessons,
  title={Lessons learned in software testing},
  author={Kaner, Cem and Bach, James and Pettichord, Bret},
  year={2008},
  publisher={John Wiley \& Sons}
}
@inproceedings{del2005improving,
	Author = {Del Grosso, Concettina and Antoniol, Giuliano and Di Penta, Massimiliano and Galinier, Philippe and Merlo, Ettore},
	Booktitle = {Proceedings of the 7th annual conference on Genetic and evolutionary computation},
	Organization = {ACM},
	Pages = {1037--1043},
	Title = {Improving network applications security: a new heuristic to generate stress testing data},
	Year = {2005}}

@article{derderian2006automated,
	Author = {Derderian, Karnig and Hierons, Robert M and Harman, Mark and Guo, Qiang},
	Journal = {The Computer Journal},
	Number = {3},
	Pages = {331--344},
	Publisher = {Br Computer Soc},
	Title = {Automated unique input output sequence generation for conformance testing of FSMs},
	Volume = {49},
	Year = {2006}}

@article{duran:1984,
	Author = {Joe W. Duran and Simeon C. Ntafos},
	Journal = {{IEEE} Trans. Software Eng.},
	Number = {4},
	Pages = {438--444},
	Title = {An Evaluation of Random Testing},
	Volume = {10},
	Year = {1984}}

@book{fenton:2014,
	Author = {Fenton, Norman and Bieman, James},
	Date-Added = {2016-03-16 09:35:22 +0000},
	Date-Modified = {2016-03-16 09:35:30 +0000},
	Publisher = {CRC Press},
	Title = {Software metrics: a rigorous and practical approach},
	Year = {2014}}

@inproceedings{fraser:2016,
	Acmid = {2897020},
	Address = {New York, NY, USA},
	Author = {Fraser, Gordon and Arcuri, Andrea},
	Booktitle = {Proceedings of the 9th International Workshop on Search-Based Software Testing},
	Date-Added = {2017-02-12 12:04:27 +0000},
	Date-Modified = {2017-02-12 12:04:38 +0000},
	Doi = {10.1145/2897010.2897020},
	Isbn = {978-1-4503-4166-0},
	Keywords = {search-based software engineering, search-based testing, test case generation, testing classes},
	Location = {Austin, Texas},
	Numpages = {4},
	Pages = {33--36},
	Publisher = {ACM},
	Series = {SBST '16},
	Title = {EvoSuite at the SBST 2016 Tool Competition},
	Url = {http://doi.acm.org/10.1145/2897010.2897020},
	Year = {2016},
	Bdsk-Url-1 = {http://doi.acm.org/10.1145/2897010.2897020},
	Bdsk-Url-2 = {http://dx.doi.org/10.1145/2897010.2897020}}

@inproceedings{fraser:2015,
	Author = {Fraser, Gordon and Arcuri, Andrea},
	Booktitle = {Proceedings of the Eighth International Workshop on Search-Based Software Testing},
	Date-Added = {2016-05-03 09:30:39 +0000},
	Date-Modified = {2016-05-03 09:30:51 +0000},
	Organization = {IEEE Press},
	Pages = {25--27},
	Title = {EvoSuite at the SBST 2015 tool competition},
	Year = {2015}}

@article{fraser:2014,
	Acmid = {2685612},
	Address = {New York, NY, USA},
	Articleno = {8},
	Author = {Fraser, Gordon and Arcuri, Andrea},
	Doi = {10.1145/2685612},
	Issn = {1049-331X},
	Journal = {ACM Transactions on Software Engineering and Methodology},
	Number = {2},
	Pages = {8:1--8:42},
	Publisher = {ACM},
	Title = {A Large-Scale Evaluation of Automated Unit Test Generation Using EvoSuite},
	Volume = {24},
	Year = {2014},}

@article{Fraser13A,
	Author = {Gordon Fraser and Andrea Arcuri},
	Issn = {0098-5589},
	Journal = {IEEE Transactions on Software Engineering},
	Number = {2},
	Pages = {276-291},
	Publisher = {IEEE Computer Society},
	Title = {Whole Test Suite Generation},
	Volume = {39},
	Year = {2013}}

@inproceedings{fraser:2011,
	Author = {Fraser, Gordon and Arcuri, Andrea},
	Booktitle = {Proceedings of the 19th ACM SIGSOFT symposium and the 13th European conference on Foundations of software engineering},
	Organization = {ACM},
	Pages = {416--419},
	Title = {Evosuite: automatic test suite generation for object-oriented software},
	Year = {2011}}

@inproceedings{ghani:2009,
	Author = {Ghani, Kamran and Clark, John A and Zhan, Yuan},
	Booktitle = {Evolutionary Computation, 2009. CEC'09. IEEE Congress on},
	Date-Added = {2016-03-16 05:59:58 +0000},
	Date-Modified = {2016-03-16 06:00:07 +0000},
	Organization = {IEEE},
	Pages = {2940--2947},
	Title = {Comparing algorithms for search-based test data generation of matlab{\textregistered} simulink{\textregistered} models},
	Year = {2009}}

@inproceedings{harman2011strong,
	Author = {Harman, Mark and Jia, Yue and Langdon, William B},
	Booktitle = {ACM SIGSOFT Symposium and European Conference on Foundations of Software Engineering},
	Organization = {ACM},
	Pages = {212--222},
	Title = {Strong higher order mutation-based test data generation},
	Year = {2011}}

@article{harman:2009,
	Author = {Harman, Mark and Mansouri, S Afshin and Zhang, Yuanyuan},
	Date-Added = {2017-02-20 09:44:04 +0000},
	Date-Modified = {2017-02-20 09:44:13 +0000},
	Journal = {Department of Computer Science, King's College London, Tech. Rep. TR-09-03},
	Title = {Search based software engineering: A comprehensive analysis and review of trends techniques and applications},
	Year = {2009}}

@article{harman2010theoretical,
	Author = {Harman, Mark and McMinn, Phil},
	Journal = {IEEE Transactions on Software Engineering},
	Number = {2},
	Pages = {226--247},
	Publisher = {IEEE},
	Title = {A theoretical and empirical study of search-based testing: Local, global, and hybrid search},
	Volume = {36},
	Year = {2010}}

@article{hooker:1995,
	Author = {John N. Hooker},
	Journal = {J. Heuristics},
	Number = {1},
	Pages = {33--42},
	Title = {Testing heuristics: We have it all wrong},
	Volume = {1},
	Year = {1995}}

@inproceedings{jamrozik:2012,
	Author = {K. Jamrozik and G. Fraser and N. Tillmann and J. De Halleux},
	Booktitle = {2012 Proceedings of the 27th IEEE/ACM International Conference on Automated Software Engineering},
	Date-Added = {2017-02-12 07:18:35 +0000},
	Date-Modified = {2017-02-12 07:18:58 +0000},
	Doi = {10.1145/2351676.2351716},
	Keywords = {program testing;DSE;Microsoft Pex tool;assertion violation;augmented dynamic symbolic execution;boundary adequacy;code contracts;logical coverage criteria;mutation adequacy;path conditions;program crash;representative test sets;Test generation;boundary values;dynamic symbolic execution;mutation testing},
	Month = {Sept},
	Pages = {254-257},
	Title = {Augmented dynamic symbolic execution},
	Year = {2012},
	Bdsk-Url-1 = {http://dx.doi.org/10.1145/2351676.2351716}}

@article{jones1998strategy,
	Author = {Jones, Bryan F and Eyres, David E and Sthamer, H-H},
	Journal = {The Computer Journal},
	Number = {2},
	Pages = {98--107},
	Publisher = {Br Computer Soc},
	Title = {A strategy for using genetic algorithms to automate branch and fault-based testing},
	Volume = {41},
	Year = {1998}}

@article{jones:1996,
	Author = {Jones, Bryan F and Sthamer, H-H and Eyres, David E},
	Date-Added = {2016-03-16 07:50:47 +0000},
	Date-Modified = {2016-03-16 07:50:55 +0000},
	Journal = {Software Engineering Journal},
	Number = {5},
	Pages = {299--306},
	Publisher = {IET},
	Title = {Automatic structural testing using genetic algorithms},
	Volume = {11},
	Year = {1996}}

@article{lammermann:2008,
	Author = {Frank Lammermann and Andr{\'e} Baresel and Joachim Wegener},
	Date-Added = {2016-03-23 02:29:35 +0000},
	Date-Modified = {2016-03-23 02:29:45 +0000},
	Doi = {http://dx.doi.org/10.1016/j.asoc.2006.06.010},
	Issn = {1568-4946},
	Journal = {Applied Soft Computing},
	Keywords = {Evolutionary testability},
	Number = {2},
	Pages = {1018 - 1028},
	Title = {Evaluating evolutionary testability for structure-oriented testing with software measurements},
	Volume = {8},
	Year = {2008},
	Bdsk-Url-1 = {http://dx.doi.org/10.1016/j.asoc.2006.06.010}}

@inproceedings{ma:2015,
	Author = {Ma, Lei and Artho, Cyrille and Zhang, Cheng and Sato, Hiroyuki and Gmeiner, Johannes and Ramler, Rudolf},
	Booktitle = {Automated Software Engineering (ASE), 2015 30th IEEE/ACM International Conference on},
	Date-Added = {2016-04-28 05:12:18 +0000},
	Date-Modified = {2016-04-28 05:14:26 +0000},
	Organization = {IEEE},
	Pages = {212--223},
	Title = {GRT: Program-Analysis-Guided Random Testing (T)},
	Year = {2015}}

@article{maheshwari:2015,
	Author = {Maheshwari, V and Prasanna, M},
	Date-Added = {2016-03-14 09:02:19 +0000},
	Date-Modified = {2016-03-14 09:03:25 +0000},
	Journal = {Indian Journal of Science and Technology},
	Number = {35},
	Pages = {1},
	Publisher = {Indian Society for Education and Environment},
	Title = {Generation of Test Case using Automation in Software Systems-A Review},
	Volume = {8},
	Year = {2015}}

@unpublished{maratmu:2005,
	Author = {Manish Maratmu},
	Date-Added = {2017-02-15 10:04:25 +0000},
	Date-Modified = {2017-02-20 10:20:51 +0000},
	Note = {developer.spikesource.com/wiki/index.php/Projects:testgen4j, last access December 2008.},
	Title = {TestGen4J}}

@article{mccabe:1976,
	Acmid = {1313586},
	Address = {Piscataway, NJ, USA},
	Author = {McCabe, T. J.},
	Date-Added = {2017-02-12 04:12:25 +0000},
	Date-Modified = {2017-02-12 04:12:37 +0000},
	Doi = {10.1109/TSE.1976.233837},
	Issn = {0098-5589},
	Issue_Date = {July 1976},
	Journal = {IEEE Trans. Softw. Eng.},
	Number = {4},
	Numpages = {13},
	Pages = {308--320},
	Publisher = {IEEE Press},
	Title = {A Complexity Measure},
	Url = {http://dx.doi.org/10.1109/TSE.1976.233837},
	Volume = {2},
	Year = {1976},
	Bdsk-Url-1 = {http://dx.doi.org/10.1109/TSE.1976.233837}}

@article{mcminn2004search,
	Author = {McMinn, Phil},
	Journal = {Software Testing Verification and Reliability},
	Number = {2},
	Pages = {105--156},
	Publisher = {Citeseer},
	Title = {Search-based software test data generation: A survey},
	Volume = {14},
	Year = {2004}}

@article{mcminn2012input,
	Author = {McMinn, Phil and Harman, Mark and Lakhotia, Kiran and Hassoun, Youssef and Wegener, Joachim},
	Journal = {IEEE Transactions on Software Engineering},
	Number = {2},
	Pages = {453--477},
	Publisher = {IEEE},
	Title = {Input domain reduction through irrelevant variable removal and its effect on local, global, and hybrid search-based structural test data generation},
	Volume = {38},
	Year = {2012}}

@article{michael2001generating,
	Author = {Michael, Christoph C. and McGraw, Gary and Schatz, Michael A},
	Journal = {IEEE transactions on software engineering},
	Number = {12},
	Pages = {1085--1110},
	Publisher = {IEEE},
	Title = {Generating software test data by evolution},
	Volume = {27},
	Year = {2001}}

@article{miller:1976,
	Author = {Miller, Webb and Spooner, David L.},
	Date-Added = {2016-03-16 07:49:05 +0000},
	Date-Modified = {2016-03-16 07:49:19 +0000},
	Journal = {IEEE Transactions on Software Engineering},
	Number = {3},
	Pages = {223},
	Publisher = {IEEE Computer Society},
	Title = {Automatic generation of floating-point test data},
	Volume = {2},
	Year = {1976}}

@inproceedings{nistor:2012,
	Acmid = {2337309},
	Address = {Piscataway, NJ, USA},
	Author = {Nistor, Adrian and Luo, Qingzhou and Pradel, Michael and Gross, Thomas R. and Marinov, Darko},
	Booktitle = {Proceedings of the 34th International Conference on Software Engineering},
	Date-Added = {2017-02-12 07:34:21 +0000},
	Date-Modified = {2017-02-12 07:34:30 +0000},
	Isbn = {978-1-4673-1067-3},
	Location = {Zurich, Switzerland},
	Numpages = {11},
	Pages = {727--737},
	Publisher = {IEEE Press},
	Series = {ICSE '12},
	Title = {BALLERINA: Automatic Generation and Clustering of Efficient Random Unit Tests for Multithreaded Code},
	Url = {http://dl.acm.org/citation.cfm?id=2337223.2337309},
	Year = {2012},
	Bdsk-Url-1 = {http://dl.acm.org/citation.cfm?id=2337223.2337309}}

@misc{cencus,
  author = {Mark Ludlow},
  title = {{IT disasters now part of modern life}},
  url = {https://www.afr.com/technology/it-disasters-now-part-of-modern-life-20160628-gptyw6},
  year = {2016}, 
  note = {[Online; accessed 11-December-2018]}
}

@misc{energy,
  author = {Gareth Hutchens},
  title = {{Software glitch to blame for blackout of extra 60,000 SA homes in heatwave}},
  url = {https://www.theguardian.com/australia-news/2017/feb/21/software-glitch-to-blame-for-blackout-of-extra-60000-sa-homes-in-heatwave},
  year = {2017}, 
  note = {[Online; accessed 11-December-2018]}
}

@article{eisenstadt1997my,
  title={My hairiest bug war stories},
  author={Eisenstadt, Marc},
  journal={Communications of the ACM},
  volume={40},
  number={4},
  pages={30--37},
  year={1997},
  publisher={ACM}
}
@misc{linesofcode,
  author = {Robert N. Charette},
  title = {{This Car Runs on Code}},
  url = {https://spectrum.ieee.org/transportation/systems/this-car-runs-on-code},
  year = {2009}, 
  note = {[Online; accessed 10-December-2018]}
}

@misc{british,
  author = {Sarah Butler},
  title = {{British Airways could face £100m compensation bill over IT meltdown}},
  url ={https://www.theguardian.com/business/2017/may/28/british-airways-faces-100m-compensation-bill-over-it-meltdown},
  year = {2017}, 
  note = {[Online; accessed 10-December-2018]}
}
@misc{failurecost,
  author = {Rogue Wave Software},
  title = {{University of Cambridge Study: Failure to Adopt Reverse Debugging Costs Global Economy \$41 Billion Annually}},
  url = {https://www.roguewave.com/company/news/2013/university-of-cambridge-reverse-debugging-study},
  year = {2013}, 
  note = {[Online; accessed 10-December-2018]}
}
@misc{digitalEconomy,
  author = {Senator the Hon Matt Canavan and the Hon Karen Andrews MP},
  title = {{Deciding our digital future}},
  url = {https://www.minister.industry.gov.au/ministers/sinodinos/media-releases/deciding-our-digital-future},
  year = {2013}, 
  note = {[Online; accessed 10-December-2018]}
}
@misc{selfdrivingcar,
  author = {Mark Harris},
  title = {{Google reports self-driving car mistakes: 272 failures and 13 near misses}},
  url = {https://www.theguardian.com/technology/2016/jan/12/google-self-driving-cars-mistakes-data-reports},
  year = {2016}, 
  note = {[Online; accessed 10-December-2018]},
}

@misc{sbserep,
  author = {Yuanyuan Zhang},
  title = {{SBSE Repository}},
  url = {http://crestweb.cs.ucl.ac.uk/resources/sbse_repository},
  year = {2018}, 
  note = {[Online; accessed 14-December-2018]},
}

@inproceedings{oriol:2012,
	Author = {M. Oriol},
	Booktitle = {2012 IEEE Fifth International Conference on Software Testing, Verification and Validation},
	Date-Added = {2017-02-11 03:49:23 +0000},
	Date-Modified = {2017-02-11 03:49:37 +0000},
	Doi = {10.1109/ICST.2012.100},
	Issn = {2159-4848},
	Keywords = {Java;fault tolerant computing;program testing;Java class;Michaelis-Menten equation;Qualitas corpus;automated random testing;faults;law evaluation;Approximation methods;Equations;Histograms;Java;Mathematical model;Runtime;Testing;automated;random;testing},
	Month = {April},
	Pages = {201-210},
	Title = {Random Testing: Evaluation of a Law Describing the Number of Faults Found},
	Year = {2012},
	Bdsk-Url-1 = {http://dx.doi.org/10.1109/ICST.2012.100}}

@inproceedings{pacheco:2007a,
	Author = {Pacheco, Carlos and Ernst, Michael D},
	Booktitle = {Companion to the 22nd ACM SIGPLAN conference on Object-oriented programming systems and applications companion},
	Date-Added = {2016-03-16 07:14:53 +0000},
	Date-Modified = {2016-03-16 07:15:06 +0000},
	Organization = {ACM},
	Pages = {815--816},
	Title = {Randoop: feedback-directed random testing for Java},
	Year = {2007}}

@inproceedings{pacheco2007randoop,
	Author = {Pacheco, Carlos and Ernst, Michael D},
	Booktitle = {Companion to the 22nd ACM SIGPLAN conference on Object-oriented programming systems and applications companion},
	Organization = {ACM},
	Pages = {815--816},
	Title = {Randoop: feedback-directed random testing for Java},
	Year = {2007}}

@inproceedings{pacheco:2007,
	Author = {Pacheco, Carlos and Lahiri, Shuvendu K and Ernst, Michael D and Ball, Thomas},
	Booktitle = {Software Engineering, 2007. ICSE 2007. 29th International Conference on},
	Date-Added = {2016-03-16 07:04:24 +0000},
	Date-Modified = {2016-03-16 07:04:34 +0000},
	Organization = {IEEE},
	Pages = {75--84},
	Title = {Feedback-directed random test generation},
	Year = {2007}}

@inproceedings{panichella:2017,
	Author = {A. Panichella and U. R. Molina},
	Booktitle = {2017 IEEE/ACM 10th International Workshop on Search-Based Software Testing (SBST)},
	Doi = {10.1109/SBST.2017.7},
	Keywords = {Java;program testing;software tools;statistical analysis;JUnit tool competitions;Java unit testing tool competition;automated JUnit testing tools;baseline human written test cases;benchmark infrastructure;statistical analysis;Benchmark testing;Complexity theory;Java;Libraries;Software;Tools;Java;automated unit testing;benchmark;mutation testing;statistical analysis;tool competition},
	Month = {May},
	Owner = {samaumeira},
	Pages = {32-38},
	Timestamp = {2017.10.12},
	Title = {Java Unit Testing Tool Competition - Fifth Round},
	Year = {2017},
	Bdsk-Url-1 = {http://dx.doi.org/10.1109/SBST.2017.7}}

@inproceedings{park:2012,
	Acmid = {2393636},
	Address = {New York, NY, USA},
	Articleno = {35},
	Author = {Park, Sangmin and Hossain, B. M. Mainul and Hussain, Ishtiaque and Csallner, Christoph and Grechanik, Mark and Taneja, Kunal and Fu, Chen and Xie, Qing},
	Booktitle = {Proceedings of the ACM SIGSOFT 20th International Symposium on the Foundations of Software Engineering},
	Doi = {10.1145/2393596.2393636},
	Isbn = {978-1-4503-1614-9},
	Keywords = {experimentation, statement coverage, testing},
	Location = {Cary, North Carolina},
	Numpages = {11},
	Pages = {35:1--35:11},
	Publisher = {ACM},
	Series = {FSE '12},
	Title = {CarFast: Achieving Higher Statement Coverage Faster},
	Url = {http://doi.acm.org/10.1145/2393596.2393636},
	Year = {2012},
	Bdsk-Url-1 = {http://doi.acm.org/10.1145/2393596.2393636},
	Bdsk-Url-2 = {http://dx.doi.org/10.1145/2393596.2393636}}

@article{polat2009novel,
	Author = {Polat, Kemal and G{\"u}ne{\c{s}}, Salih},
	Journal = {Expert Systems with Applications},
	Number = {2},
	Pages = {1587--1592},
	Publisher = {Elsevier},
	Title = {A novel hybrid intelligent method based on C4. 5 decision tree classifier and one-against-all approach for multi-class classification problems},
	Volume = {36},
	Year = {2009}}

@article{rice:1976,
	Added-At = {2011-11-29T00:00:00.000+0100},
	Author = {Rice, John R.},
	Biburl = {http://www.bibsonomy.org/bibtex/24c209757a25c1e97a3cfb73d78b90501/dblp},
	Date-Added = {2016-03-14 13:45:37 +0000},
	Date-Modified = {2016-03-14 13:45:46 +0000},
	Ee = {http://dx.doi.org/10.1016/S0065-2458(08)60520-3},
	Interhash = {4ebf9b095c555ac16a86debd79558673},
	Intrahash = {4c209757a25c1e97a3cfb73d78b90501},
	Journal = {Advances in Computers},
	Keywords = {dblp},
	Pages = {65-118},
	Timestamp = {2011-12-01T11:35:17.000+0100},
	Title = {The Algorithm Selection Problem.},
	Url = {http://dblp.uni-trier.de/db/journals/ac/ac15.html#Rice76},
	Volume = {15},
	Year = {1976},
	Bdsk-Url-1 = {http://dblp.uni-trier.de/db/journals/ac/ac15.html#Rice76}}

@inproceedings{rueda:2015,
	Author = {Rueda, Urko and Vos, Tanja EJ and Prasetya, ISWB},
	Booktitle = {Proceedings of the Eighth International Workshop on Search-Based Software Testing},
	Date-Added = {2016-04-28 05:31:44 +0000},
	Date-Modified = {2016-04-28 05:31:53 +0000},
	Organization = {IEEE Press},
	Pages = {19--24},
	Title = {Unit testing tool competition: Round three},
	Year = {2015}}

@inproceedings{schult:2008,
	Author = {Schult, Daniel A and Swart, P},
	Booktitle = {Proceedings of the 7th Python in Science Conferences (SciPy 2008)},
	Date-Added = {2017-02-12 12:50:09 +0000},
	Date-Modified = {2017-02-12 12:50:17 +0000},
	Pages = {11--16},
	Title = {Exploring network structure, dynamics, and function using NetworkX},
	Volume = {2008},
	Year = {2008}}

@article{sharma:2013,
	Author = {Sharma, Sachin and VISHAWJYOTI, Mrs},
	Date-Added = {2016-03-14 14:03:27 +0000},
	Date-Modified = {2016-03-14 14:03:37 +0000},
	Journal = {Journal of Global Research in Computer Science},
	Number = {12},
	Pages = {36--43},
	Title = {STUDY AND ANALYSIS OF AUTOMATION TESTING TECHNIQUES},
	Volume = {3},
	Year = {2013}}

@article{Smith-Miles:2009b,
	Acmid = {1456656},
	Address = {New York, NY, USA},
	Articleno = {6},
	Author = {Smith-Miles, Kate A.},
	Date-Added = {2017-02-10 02:45:46 +0000},
	Date-Modified = {2017-02-10 02:46:05 +0000},
	Doi = {10.1145/1456650.1456656},
	Issn = {0360-0300},
	Issue_Date = {January 2009},
	Journal = {ACM Computing Surveys},
	Keywords = {Algorithm selection, classification, combinatorial optimization, constraint satisfaction, dataset characterization, empirical hardness, forecasting, landscape analysis, meta-learning, model selection, sorting},
	Month = jan,
	Number = {1},
	Numpages = {25},
	Pages = {6:1--6:25},
	Publisher = {ACM},
	Title = {Cross-disciplinary Perspectives on Meta-learning for Algorithm Selection},
	Url = {http://doi.acm.org/10.1145/1456650.1456656},
	Volume = {41},
	Year = {2009},
	Bdsk-Url-1 = {http://doi.acm.org/10.1145/1456650.1456656},
	Bdsk-Url-2 = {http://dx.doi.org/10.1145/1456650.1456656}}

@article{smith-Miles:2014,
	Added-At = {2014-01-24T00:00:00.000+0100},
	Author = {Smith-Miles, Kate A. and Baatar, Davaatseren and Wreford, Brendan and Lewis, Rhyd},
	Biburl = {http://www.bibsonomy.org/bibtex/29e6e6815bf6f5a00992a6067fb07f81b/dblp},
	Date-Added = {2016-03-16 08:48:47 +0000},
	Date-Modified = {2016-03-16 08:49:03 +0000},
	Ee = {http://dx.doi.org/10.1016/j.cor.2013.11.015},
	Interhash = {70b382b238a986ee43e8b4f39998a2bd},
	Intrahash = {9e6e6815bf6f5a00992a6067fb07f81b},
	Journal = {Computers \& Operations Research},
	Keywords = {dblp},
	Pages = {12-24},
	Timestamp = {2014-01-25T11:33:26.000+0100},
	Title = {Towards objective measures of algorithm performance across instance space.},
	Url = {http://dblp.uni-trier.de/db/journals/cor/cor45.html#Smith-MilesBWL14},
	Volume = {45},
	Year = {2014},
	Bdsk-Url-1 = {http://dblp.uni-trier.de/db/journals/cor/cor45.html#Smith-MilesBWL14}}

@article{smith-Miles:2011b,
	Author = {Smith-Miles, Kate A. and van Hemert, Jano},
	Date-Added = {2016-03-16 08:49:55 +0000},
	Date-Modified = {2016-03-16 08:50:07 +0000},
	Doi = {10.1007/s10472-011-9230-5},
	Issn = {1012-2443},
	Journal = {Annals of Mathematics and Artificial Intelligence},
	Keywords = {Algorithm selection; Combinatorial optimization; Travelling salesman problem; Hardness prediction; Phase transition; Instance difficulty; 49-04; 68Q25; 68Q87; 68T05; 68T20; 90B99},
	Language = {English},
	Number = {2},
	Pages = {87-104},
	Publisher = {Springer Netherlands},
	Title = {Discovering the suitability of optimisation algorithms by learning from evolved instances},
	Url = {http://dx.doi.org/10.1007/s10472-011-9230-5},
	Volume = {61},
	Year = {2011},
	Bdsk-Url-1 = {http://dx.doi.org/10.1007/s10472-011-9230-5}}

@incollection{smith-Miles:2009,
	Author = {Smith-Miles, Kate A. and James, Ross J.W. and Giffin, John W. and Tu, Yiqing},
	Booktitle = {Learning and Intelligent Optimization},
	Date-Added = {2016-03-16 08:49:55 +0000},
	Date-Modified = {2016-03-16 08:50:02 +0000},
	Doi = {10.1007/978-3-642-11169-3_7},
	Editor = {St{\"u}tzle, Thomas},
	Isbn = {978-3-642-11168-6},
	Keywords = {Scheduling; heuristics; algorithm selection; self-organizing map; performance prediction; knowledge discovery},
	Language = {English},
	Pages = {89-103},
	Publisher = {Springer Berlin Heidelberg},
	Series = {Lecture Notes in Computer Science},
	Title = {A Knowledge Discovery Approach to Understanding Relationships between Scheduling Problem Structure and Heuristic Performance},
	Url = {http://dx.doi.org/10.1007/978-3-642-11169-3_7},
	Volume = {5851},
	Year = {2009},
	Bdsk-Url-1 = {http://dx.doi.org/10.1007/978-3-642-11169-3_7}}

@incollection{smith-Miles:2011c,
	Author = {Smith-Miles, Kate A and Lopes, Leo},
	Booktitle = {Learning and Intelligent Optimization},
	Editor = {Coello, Carlos A. Coello},
	Isbn = {978-3-642-25565-6},
	Keywords = {Algorithm Selection; Timetabling; Hardness Prediction; Phase Transition; Combinatorial optimisation; Instance Difficulty},
	Language = {English},
	Pages = {524-538},
	Publisher = {Springer Berlin Heidelberg},
	Series = {Lecture Notes in Computer Science},
	Title = {Generalising Algorithm Performance in Instance Space: A Timetabling Case Study},
	Volume = {6683},
	Year = {2011}}

@inproceedings{smith-Miles:2012,
	Author = {Smith-Miles, K. and Tan, T.T.},
	Booktitle = {Evolutionary Computation (CEC), 2012 IEEE Congress on},
	Date-Added = {2016-03-14 13:46:33 +0000},
	Date-Modified = {2016-03-14 13:46:39 +0000},
	Doi = {10.1109/CEC.2012.6252992},
	Keywords = {optimisation;travelling salesman problems;algorithm footprint measurement;algorithm performance;high-dimensional feature space;instance space;instance visualization;operations research literature;optimization algorithms;traveling salesman problem;Algorithm design and analysis;Cities and towns;Extraterrestrial measurements;Optimization;Prediction algorithms;Visualization;algorithm footprints;heuristics;instance difficulty;performance metrics;traveling salesman problem},
	Month = {June},
	Pages = {1-8},
	Title = {Measuring algorithm footprints in instance space},
	Year = {2012},
	Bdsk-Url-1 = {http://dx.doi.org/10.1109/CEC.2012.6252992}}

@unpublished{spinellis:2011,
	Author = {Diomidis Spinellis and Marian Jureczko},
	Date-Added = {2017-02-20 10:15:56 +0000},
	Date-Modified = {2017-02-20 10:26:10 +0000},
	Note = {Online, 2011. http://gromit.iiar.pwr.wroc.pl/p\_inf/ckjm/, last change: May 06, 2011 5:05 pm},
	Title = {CKJM extended - An extended version of Tool for Calculating Chidamber and Kemerer Java Metrics}}

@article{srivastava2009application,
	Author = {Srivastava, Praveen Ranjan and Kim, Tai-hoon},
	Journal = {International Journal of software Engineering and its Applications},
	Number = {4},
	Pages = {87--96},
	Title = {Application of genetic algorithm in software testing},
	Volume = {3},
	Year = {2009}}

@inproceedings{tonella2004evolutionary,
	Author = {Tonella, Paolo},
	Booktitle = {ACM SIGSOFT Software Engineering Notes},
	Number = {4},
	Organization = {ACM},
	Pages = {119--128},
	Title = {Evolutionary testing of classes},
	Volume = {29},
	Year = {2004}}

@inproceedings{tracey:1998,
	Author = {Tracey, Nigel and Clark, John and Mander, Keith and McDermid, John},
	Booktitle = {Automated Software Engineering, 1998. Proceedings. 13th IEEE International Conference on},
	Date-Added = {2016-03-16 07:49:59 +0000},
	Date-Modified = {2016-03-16 07:50:06 +0000},
	Organization = {IEEE},
	Pages = {285--288},
	Title = {An automated framework for structural test-data generation},
	Year = {1998}}

@unpublished{tyborowski:2002,
	Author = {Mark Tyborowsky},
	Date-Added = {2017-02-15 10:08:52 +0000},
	Date-Modified = {2017-02-15 10:10:09 +0000},
	Note = {Online, 2002. http://jub.sourceforge.net/, last access December 2008.},
	Title = {JUB (JUnit test case Builder)}}

@inproceedings{walcott2006timeaware,
	Author = {Walcott, Kristen R and Soffa, Mary Lou and Kapfhammer, Gregory M and Roos, Robert S},
	Booktitle = {Proceedings of the 2006 international symposium on Software testing and analysis},
	Organization = {ACM},
	Pages = {1--12},
	Title = {Timeaware test suite prioritization},
	Year = {2006}}

@inproceedings{wang:2009,
	Author = {Wang, Shuang and Offutt, Jeff},
	Booktitle = {Software Testing, Verification and Validation Workshops, 2009. ICSTW'09. International Conference on},
	Date-Added = {2016-03-23 02:36:01 +0000},
	Date-Modified = {2016-03-23 02:36:09 +0000},
	Organization = {IEEE},
	Pages = {210--219},
	Title = {Comparison of unit-level automated test generation tools},
	Year = {2009}}

@inproceedings{wegener2004evaluation,
	Author = {Wegener, Joachim and B{\"u}hler, Oliver},
	Booktitle = {Genetic and Evolutionary Computation Conference},
	Organization = {Springer},
	Pages = {1400--1412},
	Title = {Evaluation of different fitness functions for the evolutionary testing of an autonomous parking system},
	Year = {2004}}
@inproceedings{FIFVerify,
 author = {Mark Harman, Peter O'Hearn},
 title = {From Start-ups to Scale-ups: Opportunities and Open Problems for Static and Dynamic Program Analysis},
 booktitle = {IEEE International Working Conference on Source Code Analysis and Manipulation},
 year = {2018},
 pages = {1--23},
 }
@article{wegener1998verifying,
	Author = {Wegener, Joachim and Grochtmann, Matthias},
	Journal = {Real-Time Systems},
	Number = {3},
	Pages = {275--298},
	Publisher = {Springer},
	Title = {Verifying timing constraints of real-time systems by means of evolutionary testing},
	Volume = {15},
	Year = {1998}}

@article{white1980domain,
	Author = {White, Lee J and Cohen, Edward I},
	Journal = {IEEE Transactions on Software Engineering},
	Number = {3},
	Pages = {247--257},
	Publisher = {IEEE},
	Title = {A domain strategy for computer program testing},
	Year = {1980}}

@article{wolpert1997no,
	Author = {Wolpert, David H and Macready, William G},
	Journal = {IEEE Transactions on Evolutionary Computation},
	Number = {1},
	Pages = {67--82},
	Publisher = {IEEE},
	Title = {No free lunch theorems for optimization},
	Volume = {1},
	Year = {1997}}

@inproceedings{yoo2009clustering,
	Author = {Yoo, Shin and Harman, Mark and Tonella, Paolo and Susi, Angelo},
	Booktitle = {Proceedings of the eighteenth international symposium on Software testing and analysis},
	Organization = {ACM},
	Pages = {201--212},
	Title = {Clustering test cases to achieve effective and scalable prioritisation incorporating expert knowledge},
	Year = {2009}}

@inproceedings{zhan:2006,
	Author = {Zhan, Yuan and Clark, John A},
	Booktitle = {Proceedings of the 8th annual conference on Genetic and evolutionary computation},
	Date-Added = {2017-03-13 06:29:12 +0000},
	Date-Modified = {2017-03-13 06:29:21 +0000},
	Organization = {ACM},
	Pages = {1941--1948},
	Title = {The state problem for test generation in simulink},
	Year = {2006}}

@inproceedings{zhan2005search,
	Author = {Zhan, Yuan and Clark, John A},
	Booktitle = {Proceedings of the 7th annual conference on Genetic and evolutionary computation},
	Organization = {ACM},
	Pages = {1061--1068},
	Title = {Search-based mutation testing for simulink models},
	Year = {2005}}

@inproceedings{zhang:2011,
	Author = {Sai Zhang and David Saff and Yingyi Bu and and Michael D. Ernst},
	Booktitle = {Proc. 11th International Symposium on Software Testing and Analysis (ISSTA 2011)},
	Date-Added = {2017-02-15 11:45:35 +0000},
	Date-Modified = {2017-02-15 11:45:50 +0000},
	Location = {Toronto, ON, Canada},
	Title = {Combined Static and Dynamic Automated Test Generation},
	Year = {2011}}

@article{LeGoues2013current,
  title={Current challenges in automatic software repair},
  author={Le Goues, Claire and Forrest, Stephanie and Weimer, Westley},
  journal={Software Quality Journal},
  volume={21},
  number={3},
  pages={421--443},
  year={2013},
  publisher={Springer},
  doi       = {10.1007/s11219-013-9208-0},

}
@inproceedings{Weimer2009GFPatches,
 author = {Weimer, Westley and Nguyen, ThanhVu and Le Goues, Claire and Forrest, Stephanie},
 title = {Automatically Finding Patches Using Genetic Programming},
 booktitle = {International Conference on Software Engineering},
 series = {ICSE},
 year = {2009},
 isbn = {978-1-4244-3453-4},
 pages = {364--374},
 numpages = {11},
   url       = {http://dx.doi.org/10.1109/ICSE.2009.5070536},
  doi       = {10.1109/ICSE.2009.5070536},

}
@article{LeGoues2012GenProg,
 title={GenProg: A generic method for automatic software repair},
  author={Le Goues, Claire and Nguyen, ThanhVu and Forrest, Stephanie and Weimer, Westley},
  journal={Software Engineering, IEEE Transactions on},
  volume={38},
  number={1},
  pages={54--72},
  year={2012},
  publisher={IEEE},
  doi       = {10.1109/TSE.2011.104},
}
@inproceedings{LeGoues2012Study,
 author = {Le Goues, Claire and Dewey-Vogt, Michael and Forrest, Stephanie and Weimer, Westley},
 title = {A Systematic Study of Automated Program Repair: Fixing 55 out of 105 Bugs for \$8 Each},
 booktitle = {International Conference on Software Engineering},
  doi       = {10.1109/ICSE.2012.6227211},
 series = {ICSE},
 year = {2012},
 isbn = {978-1-4673-1067-3},
 _location = {Zurich, Switzerland},
 pages = {3--13},
 numpages = {11},
 publisher = {IEEE Press},
 _address = {Piscataway, NJ, USA},
}
@article{DurieuxMMSX15,
  author    = {Thomas Durieux and
               Matias Martinez and
               Martin Monperrus and
               Romain Sommerard and
               Jifeng Xuan},
  title     = {Automatic Repair of Real Bugs: An Experience Report on the Defects4J
               Dataset},
  journal   = {CoRR},
  volume    = {abs/1505.07002},
  year      = {2015},
}

@article{MartinezM15,
  author    = {Matias Martinez and
               Martin Monperrus},
  title     = {Mining software repair models for reasoning on the search space of
               automated program fixing},
  journal   = {Empirical Software Engineering},
  volume    = {20},
  number    = {1},
  pages     = {176--205},
  year      = {2015},
  doi       = {10.1007/s10664-013-9282-8},

}
@ARTICLE{Xuan16MDCLDLM,
  author    = {Jifeng Xuan and
               Matias Martinez and
               Favio Demarco and
               Maxime Clement and
               Sebastian R. Lamelas Marcote and
               Thomas Durieux and
               Daniel Le Berre and
               Martin Monperrus},
  title     = {Nopol: Automatic Repair of Conditional Statement Bugs in Java Programs},
  journal   = {{IEEE} Transactions Software Engineering},
  volume    = {43},
  number    = {1},
  pages     = {34--55},
  year      = {2017},
  doi       = {10.1109/TSE.2016.2560811},
}
@inproceedings{Kim13PAR,
 author = {Kim, Dongsun and Nam, Jaechang and Song, Jaewoo and Kim, Sunghun},
 title = {Automatic Patch Generation Learned from Human-written Patches},
 booktitle = {International Conference on Software Engineering},
 year = {2013},
 isbn = {978-1-4673-3076-3},
 pages = {802--811},
 numpages = {10},
 publisher = {IEEE Press},
  doi       = {10.1109/ICSE.2013.6606626},
}
@article{McMinn04,
author = {Phil McMinn},
title = {Search-based Software Test Data Generation: A Survey},
journal = {Software Testing, Verification and Reliability},
volume = {14},
number = {2},
pages = {105â156},
year = {2004},
}
@InProceedings{Harman07PC,
  author =	"Mark Harman",
  title =	"Search Based Software Engineering for Program Comprehension",
  booktitle =	"Int. Conf. on Program Comprehension (ICPC 2007)",
  year = 	"2007",
  note = 	"Invited paper",
  publisher =	"IEEE",
}
@InProceedings{Harman07,
  title =	"The Current State and Future of Search Based Software
		 Engineering",
  author =	"Mark Harman",
  booktitle =	"International Conference on Software Engineering,
		 {ISCE}, Workshop on the Future of Software Engineering",
  year = 	"2007",
  _editor =	"Lionel C. Briand and Alexander L. Wolf",
  pages =	"342--357",
}
@article{FraserA15,
  author    = {Gordon Fraser and
               Andrea Arcuri},
  title     = {1600 faults in 100 projects: automatically finding faults while achieving
               high coverage with EvoSuite},
  journal   = {Empirical Software Engineering},
  volume    = {20},
  number    = {3},
  pages     = {611--639},
  year      = {2015},
}
@inproceedings{KimXKCR14,
  author    = {Yunho Kim and
               Zhihong Xu and
               Moonzoo Kim and
               Myra B. Cohen and
               Gregg Rothermel},
  title     = {Hybrid Directed Test Suite Augmentation: An Interleaving Framework},
  booktitle = {Seventh {IEEE} International Conference on Software Testing, Verification
               and Validation, {ICST}},
  pages     = {263--272},
  publisher = {{IEEE} Computer Society},
  year      = {2014},
}
@inproceedings{XuKKR11,
  author    = {Zhihong Xu and
               Yunho Kim and
               Moonzoo Kim and
               Gregg Rothermel},
  title     = {A Hybrid Directed Test Suite Augmentation Technique},
  booktitle = {{IEEE} 22nd International Symposium on Software Reliability Engineering},
  pages     = {150--159},
  publisher = {{IEEE} Computer Society},
  year      = {2011},
}
@article{XuKKCR15,
  author    = {Zhihong Xu and
               Yunho Kim and
               Moonzoo Kim and
               Myra B. Cohen and
               Gregg Rothermel},
  title     = {Directed test suite augmentation: an empirical investigation},
  journal   = {Softw. Test., Verif. Reliab.},
  volume    = {25},
  number    = {2},
  pages     = {77--114},
  year      = {2015},
}
@article{YooH12,
  author    = {Shin Yoo and
               Mark Harman},
  title     = {Regression testing minimization, selection and prioritization: a survey},
  journal   = {Softw. Test., Verif. Reliab.},
  volume    = {22},
  number    = {2},
  pages     = {67--120},
  year      = {2012},
}
@Article{FraserAM15,
  title =	"A Memetic Algorithm for whole test suite generation",
  author =	"Gordon Fraser and Andrea Arcuri and Phil McMinn",
  journal =	"Journal of Systems and Software",
  year = 	"2015",
  volume =	"103",
  pages =	"311--327",
}
@Article{MaoXYC15,
  title =	"Adapting ant colony optimization to generate test data
		 for software structural testing",
  author =	"Chengying Mao and Lichuan Xiao and Xinxin Yu and Jinfu
		 Chen",
  journal =	"Swarm and Evolutionary Computation",
  year = 	"2015",
  volume =	"20",
  pages =	"23--36",
}
@Article{Merz00F,
    author =	{Peter Merz and Bernd Freisleben},
    title =	{Fitness Landscape Analysis and Memetic Algorithms for the Quadratic Assignment Problem},
    journal =	{IEEE Evolutionary Computation},
    volume =	{4},
    number =	{4},
    pages =	{337-352},
	year = 	{2000},
}
@Article{SmithHLO02,
  title =	"Fitness Landscapes and Evolvability",
  author =	"Tom Smith and Phil Husbands and Paul J. Layzell and
		 Michael O'Shea",
  journal =	"Evolutionary Computation",
  year = 	"2002",
  number =	"1",
  volume =	"10",
  pages =	"1--34",
}
@Article{Weinberger91b,
    author =	{Edward D. Weinberger},
    title =	{Local Properties of Kauffman's {N}-k model: {A} tunably Rugged Enegy Landscape},
    journal = {Physical Review A},
    volume =	{44},
    number =	{10},
    pages =	{6399--6413},
    year = 	{1991},
}
@article{Stadler96,
   author = {Peter Stadler},
   title = {Landscapes and Their Correlation Functions},
   journal = {Journal of Mathematical Chemistry},
   pages = {1--45},
   volume = {20},
   year = {1996},
}
@ARTICLE{Angel98,
    author = {Eric Angel and Vassilis Zissimopoulos},
    title = {Autocorrelation Coefficient for the Graph Bipartitioning Problem},
    journal = {Theoretical Computer Science},
    year = {1998},
    volume = {191},
    pages = {229--243}
}
@article{guyon2003introduction,
  title={An introduction to variable and feature selection},
  author={Guyon, Isabelle and Elisseeff, Andr{\'e}},
  journal={Journal of machine learning research},
  volume={3},
  number={Mar},
  pages={1157--1182},
  year={2003}
}
@article{bengio2003extensions,
  title={Extensions to metric-based model selection},
  author={Bengio, Yoshua and Chapados, Nicolas},
  journal={Journal of Machine Learning Research},
  volume={3},
  number={Mar},
  pages={1209--1227},
  year={2003}
}
@article{aleti2014choosing,
  title={Choosing the appropriate forecasting model for predictive parameter control},
  author={Aleti, Aldeida and Moser, Irene and Meedeniya, Indika and Grunske, Lars},
  journal={Evolutionary computation},
  volume={22},
  number={2},
  pages={319--349},
  year={2014},
  publisher={MIT Press}
}
@Article{Yu2019Alleviating,
author="Yu, Zhongxing
and Martinez, Matias
and Danglot, Benjamin
and Durieux, Thomas
and Monperrus, Martin",
title="Alleviating patch overfitting with automatic test generation: a study of feasibility and effectiveness for the Nopol repair system",
journal="Empirical Software Engineering",
year="2019",
month="Feb",
day="01",
volume="24",
number="1",
pages="33--67",
issn="1573-7616",
doi="10.1007/s10664-018-9619-4",
}
@article{Yuan2018ARJA,
    author = {Yuan, Yuan and Banzhaf, Wolfgang},
    title = {{ARJA: Automated Repair of Java Programs via Multi-Objective Genetic Programming}},
    journal = {IEEE Transactions on Software Engineering},
    year = {2018},
    month = {},
    pages = {},
    volume = {PP},
    doi = {10.1109/TSE.2018.2874648},
}
@book{jolliffe2011principal,
  title={Principal component analysis},
  author={Jolliffe, Ian},
  year={2011},
  publisher={Springer}
}

@inproceedings{Long2016prophet,
author = {Long, Fan and Rinard, Martin},
title = {Automatic Patch Generation by Learning Correct Code},
year = {2016},
isbn = {9781450335492},
publisher = {Association for Computing Machinery},
address = {New York, NY, USA},
url = {https://doi.org/10.1145/2837614.2837617},
doi = {10.1145/2837614.2837617},
booktitle = {Proceedings of the 43rd Annual ACM SIGPLAN-SIGACT Symposium on Principles of Programming Languages},
pages = {298–312},
numpages = {15},
keywords = {Learning correct code, Code correctness model, Program repair},
location = {St. Petersburg, FL, USA},
series = {POPL ’16}
}
@inproceedings{Long2015SPR,
author = {Long, Fan and Rinard, Martin},
title = {Staged Program Repair with Condition Synthesis},
year = {2015},
isbn = {9781450336758},
publisher = {Association for Computing Machinery},
address = {New York, NY, USA},
url = {https://doi.org/10.1145/2786805.2786811},
doi = {10.1145/2786805.2786811},
booktitle = {Proceedings of the 2015 10th Joint Meeting on Foundations of Software Engineering},
pages = {166--178},
numpages = {13},
keywords = {Program repair, Staged repair, Condition synthesis},
location = {Bergamo, Italy},
series = {ESEC/FSE 2015},
}
  
@article{smith2014towards,
  title={Towards objective measures of algorithm performance across instance space},
  author={Smith-Miles, Kate and Baatar, Davaatseren and Wreford, Brendan and Lewis, Rhyd},
  journal={Computers \& Operations Research},
  volume={45},
  pages={12--24},
  year={2014},
  publisher={Elsevier}
}

@inproceedings{el2004object,
  title={Object-oriented design quality models a survey and comparison},
  author={El-Wakil, Mohamed and El-Bastawisi, Ali and Boshra, Mokhtar and Fahmy, Ali},
  booktitle={2nd International Conference on Informatics and Systems},
  pages={1--11},
  year={2004}
}

@inproceedings{Durieux:2019:RepairThemAll,
 author = {Durieux, Thomas and Madeiral, Fernanda and Martinez, Matias and Abreu, Rui},
 title = {Empirical Review of Java Program Repair Tools: A Large-scale Experiment on 2,141 Bugs and 23,551 Repair Attempts},
 booktitle = {Proceedings of the 2019 27th ACM Joint Meeting on European Software Engineering Conference and Symposium on the Foundations of Software Engineering},
 year = {2019},
 isbn = {978-1-4503-5572-8},
 pages = {302--313},
 doi = {10.1145/3338906.3338911},
 publisher = {ACM},
} 

@misc{1906.03447,
Author = {Shangwen Wang and Ming Wen and Liqian Chen and Xin Yi and Xiaoguang Mao},
Title = {How Different Is It Between Machine-Generated and Developer-Provided Patches? An Empirical Study on The Correct Patches Generated by Automated Program Repair Techniques},
Year = {2019},
Eprint = {arXiv:1906.03447},
}

%Survey papers beginning

@article{Monperrus2018bibliography,
    author = {Monperrus, Martin},
    title = {{Automatic Software Repair: a Bibliography}},
    journal = {ACM Computing Surveys},
    issue_date = {April 2018},
    volume = {51},
    number = {1},
    month = jan,
    year = {2018},
    issn = {0360-0300},
    pages = {17:1--17:24},
    articleno = {17},
    numpages = {24},
    url = {http://doi.acm.org/10.1145/3105906},
    doi = {10.1145/3105906},
    acmid = {3105906},
    publisher = {ACM},
    address = {New York, NY, USA},
    keywords = {Program repair, self-healing software},
}

@article{Gazzola2019survey,
    author = {L. Gazzola and D. Micucci and L. Mariani},
    title = {{Automatic Software Repair: A Survey}},
    journal = {IEEE Transactions on Software Engineering},
    volume = {45},
    number = {1},
    month = jan,
    year = {2019},
    issn = {0098-5589},
    pages = {34--67},
    doi = {10.1109/TSE.2017.2755013},
    publisher = {IEEE},
}

@article{Liu2018survey,
    author = {Yuzhen Liu and Long Zhang and Zhenyu Zhang},
    title = {{A Survey of Test Based Automatic Program Repair}},
    journal = {Journal of Software},
    issue_date = {August 2018},
    volume = {13},
    number = {8},
    month = aug,
    year = {2018},
    issn = {1796-217X},
    pages = {437--452},
    doi = {10.17706/jsw.13.8.437-452},
}

@techreport{Monperrus2018living,
    author = {Martin Monperrus},
    title = {{The Living Review on Automated Program Repair}},
    number = {hal-01956501},
    institution = {HAL/archives-ouvertes.fr},
    address = {HAL/archives-ouvertes.fr},
    year = {2018}
}

%Survey papers end

%Position papers beginning

@inproceedings{Monperrus2014,
    author = {Monperrus, Martin},
    title = {{A Critical Review of ``Automatic Patch Generation Learned from Human-Written Patches'': Essay on the Problem Statement and the Evaluation of Automatic Software Repair}},
    booktitle = {Proceedings of the 36th International Conference on Software Engineering (ICSE '14)},
    year = {2014},
    isbn = {978-1-4503-2756-5},
    location = {Hyderabad, India},
    pages = {234--242},
    numpages = {9},
    url = {http://doi.acm.org/10.1145/2568225.2568324},
    doi = {10.1145/2568225.2568324},
    acmid = {2568324},
    publisher = {ACM},
    address = {New York, NY, USA},
    keywords = {Bugs, automatic patch generation, automatic program fixing, automatic software repair, error recovery, faults},
}

%Position papers end

%Repair tools beginning

@inproceedings{Xiong2017ACS,
    author = {Xiong, Yingfei and Wang, Jie and Yan, Runfa and Zhang, Jiachen and Han, Shi and Huang, Gang and Zhang, Lu},
    title = {{Precise Condition Synthesis for Program Repair}},
    booktitle = {Proceedings of the 39th International Conference on Software Engineering (ICSE '17)},
    year = {2017},
    isbn = {978-1-5386-3868-2},
    location = {Buenos Aires, Argentina},
    pages = {416--426},
    numpages = {11},
    doi = {10.1109/ICSE.2017.45},
    acmid = {3097418},
    publisher = {IEEE Press},
}

@inproceedings{Wen2018CapGen,
    author = {Wen, Ming and Chen, Junjie and Wu, Rongxin and Hao, Dan and Cheung, Shing-Chi},
    title = {{Context-Aware Patch Generation for Better Automated Program Repair}},
    booktitle = {International Conference on Software Engineering},
    year = {2018},
    isbn = {978-1-4503-5638-1},
    pages = {1--11},
    doi = {10.1145/3180155.3180233},
    acmid = {3180233},
    publisher = {ACM},
} 

@inproceedings{Martinez2018Cardumen,
    author = {Martinez, Matias and Monperrus, Martin},
    editor = {Colanzi, Thelma Elita and McMinn, Phil},
    title = {{Ultra-Large Repair Search Space with Automatically Mined Templates: the Cardumen Mode of Astor}},
    booktitle = {International Symposium on Search-Based Software Engineering. Lecture Notes in Computer Science, vol 11036},
    year = {2018},
    isbn = {978-3-319-99241-9},
    pages = {65--86},
    publisher = {Springer},
}

@inproceedings{White2019DeepRepair,
    author = {White, Martin and Tufano, Michele and Martinez, Matias and Monperrus, Martin and Poshyvanyk, Denys},
    title = {{Sorting and Transforming Program Repair Ingredients via Deep Learning Code Similarities}},
    booktitle = {IEEE International Conference on Software Analysis, Evolution and Reengineering},
    year = {2019},
    pages = {479--490},
    publisher = {IEEE},
}

@inproceedings{Durieux2016DynaMoth,
    author = {Durieux, Thomas and Monperrus, Martin},
    title = {{DynaMoth: Dynamic Code Synthesis for Automatic Program Repair}},
    booktitle = {International Workshop on Automation of Software Test},
    year = {2016},
    isbn = {978-1-4503-4151-6},
    pages = {85--91},
    doi = {10.1145/2896921.2896931},
    acmid = {2896931},
    publisher = {ACM},
} 

@inproceedings{Saha2017ELIXIR,
    author = {Saha, Ripon K. and Lyu, Yingjun and Yoshida, Hiroaki and Prasad, Mukul R.},
    title = {{ELIXIR: Effective Object-Oriented Program Repair}},
    booktitle = {IEEE/ACM International Conference on Automated Software Engineering},
    year = {2017},
    isbn = {978-1-5386-2684-9},
    pages = {648--659},
    acmid = {3155643},
    publisher = {IEEE Press},
} 

@inproceedings{Le2016HDRepair,
    author = {Le, Xuan Bach D. and Lo, David and {Le Goues}, Claire},
    title = {{History Driven Program Repair}},
    booktitle = {International Conference on Software Analysis, Evolution and Reengineering},
    year = {2016},
    isbn = {978-1-5090-1855-0},
    pages = {213--224},
    doi = {10.1109/SANER.2016.76},
    publisher = {IEEE},
}

@inproceedings{Chen2017Jaid,
    author = {Chen, Liushan and Pei, Yu and Furia, Carlo A.},
    title = {{Contract-Based Program Repair without the Contracts}},
    booktitle = {IEEE/ACM International Conference on Automated Software Engineering},
    year = {2017},
    isbn = {978-1-5386-2684-9},
    pages = {637--647},
    acmid = {3155642},
    publisher = {IEEE Press},
} 

@inproceedings{Martinez2016Astor,
    author = {Martinez, Matias and Monperrus, Martin},
    title = {{ASTOR: A Program Repair Library for Java}},
    booktitle = {Proceedings of the 25th International Symposium on Software Testing and Analysis, Demonstration Track},
    year = {2016},
    isbn = {978-1-4503-4390-9},
    pages = {441--444},
    doi = {10.1145/2931037.2948705},
    acmid = {2948705},
    publisher = {ACM},
}

@inproceedings{Liu2018LSRepair,
    author = {Liu, Kui and Koyuncu, Anil and Kim, Kisub and Kim, Dongsun and F. Bissyand{\'e}, Tegawend{\'e}},
    title = {{LSRepair: Live Search of Fix Ingredients for Automated Program Repair}},
    booktitle = {Asia-Pacific Software Engineering Conference},
    year = {2018},
    pages = {1--5},
    publisher = {IEEE Computer Society},
    address = {Washington, DC, USA},
}

@inproceedings{Durieux2017NPEFix,
    author = {Durieux, Thomas and Cornu, Benoit and Seinturier, Lionel and Monperrus, Martin},
    title = {{Dynamic Patch Generation for Null Pointer Exceptions Using Metaprogramming}},
    booktitle = {Proceedings of the 24th IEEE International Conference on Software Analysis, Evolution and Reengineering (SANER '17)},
    year = {2017},
    pages = {349--358},
    doi = {10.1109/SANER.2017.7884635},
    publisher = {IEEE},
}

@inproceedings{Kim2013PAR,
    author = {Kim, Dongsun and Nam, Jaechang and Song, Jaewoo and Kim, Sunghun},
    title = {{Automatic Patch Generation Learned from Human-Written Patches}},
    booktitle = {International Conference on Software Engineering (ICSE '13)},
    year = {2013},
    isbn = {978-1-4673-3076-3},
    pages = {802--811},
    acmid = {2486893},
    publisher = {IEEE Press},
}

@inproceedings{Jiang2018SimFix,
    author = {Jiang, Jiajun and Xiong, Yingfei and Zhang, Hongyu and Gao, Qing and Chen, Xiangqun},
    title = {{Shaping Program Repair Space with Existing Patches and Similar Code}},
    booktitle = {Proceedings of the 27th ACM SIGSOFT International Symposium on Software Testing and Analysis (ISSTA '18)},
    year = {2018},
    isbn = {978-1-4503-5699-2},
    pages = {298--309},
    doi = {10.1145/3213846.3213871},
    acmid = {3213871},
    publisher = {ACM},
}

@inproceedings{Hua2018SketchFix,
    author = {Hua, Jinru and Zhang, Mengshi and Wang, Kaiyuan and Khurshid, Sarfraz},
    title = {{Towards Practical Program Repair with On-Demand Candidate Generation}},
    booktitle = {International Conference on Software Engineering},
    year = {2018},
    isbn = {978-1-4503-5638-1},
    pages = {12--23},
    url = {http://doi.acm.org/10.1145/3180155.3180245},
    doi = {10.1145/3180155.3180245},
    acmid = {3180245},
    publisher = {ACM},
    address = {New York, NY, USA},
}

@inproceedings{Liu2018SOFix,
    author = {Xuliang Liu and Hao Zhong},
    title = {{Mining StackOverflow for Program Repair}},
    booktitle = {Proceedings of the 25th IEEE International Conference on Software Analysis, Evolution and Reengineering (SANER '18)},
    year = {2018},
    location = {Campobasso, Italy},
    pages = {118--129},
    numpages = {12},
    doi = {10.1109/SANER.2018.8330202},
    publisher = {IEEE},
    address = {Campobasso, Italy},
}

@inproceedings{Xin2017ssFix,
    author = {Xin, Qi and Reiss, Steven P.},
    title = {{Leveraging Syntax-Related Code for Automated Program Repair}},
    booktitle = {Proceedings of the 32nd IEEE/ACM International Conference on Automated Software Engineering (ASE '17)},
    year = {2017},
    isbn = {978-1-5386-2684-9},
    location = {Urbana-Champaign, IL, USA},
    pages = {660--670},
    numpages = {11},
    url = {http://dl.acm.org/citation.cfm?id=3155562.3155644},
    acmid = {3155644},
    publisher = {IEEE Press},
    address = {Piscataway, NJ, USA},
    keywords = {Automated program repair, code search, code transfer},
}

@inproceedings{Weimer2009GenProg,
    author = {Weimer, Westley and Nguyen, ThanhVu and {Le Goues}, Claire and Forrest, Stephanie},
    title = {{Automatically Finding Patches Using Genetic Programming}},
    booktitle = {Proceedings of the 31st International Conference on Software Engineering},
    year = {2009},
    isbn = {978-1-4244-3453-4},
    pages = {364--374},
    acmid = {1555051},
    publisher = {IEEE Computer Society},
}

@inproceedings{Qi2015Kali,
    author = {Qi, Zichao and Long, Fan and Achour, Sara and Rinard, Martin},
    title = {{An Analysis of Patch Plausibility and Correctness for Generate-and-Validate Patch Generation Systems}},
    booktitle = {Proceedings of the 2015 International Symposium on Software Testing and Analysis (ISSTA '15)},
    year = {2015},
    isbn = {978-1-4503-3620-8},
    location = {Baltimore, MD, USA},
    pages = {24--36},
    doi = {10.1145/2771783.2771791},
    acmid = {2771791},
    publisher = {ACM},
}

@inproceedings{Debroy2010MutRepair,
    author = {Debroy, Vidroha and Wong, W. Eric},
    title = {{Using Mutation to Automatically Suggest Fixes for Faulty Programs}},
    booktitle = {Proceedings of the 2010 Third International Conference on Software Testing, Verification and Validation (ICST '10)},
    year = {2010},
    isbn = {978-0-7695-3990-4},
    pages = {65--74},
    numpages = {10},
    url = {http://dx.doi.org/10.1109/ICST.2010.66},
    doi = {10.1109/ICST.2010.66},
    acmid = {1828445},
    publisher = {IEEE Computer Society},
    address = {Washington, DC, USA},
    keywords = {program debugging, mutation, fault localization, fault-fixing, software testing},
}

@inproceedings{Qi2014RSRepair,
    author = {Qi, Yuhua and Mao, Xiaoguang and Lei, Yan and Dai, Ziying and Wang, Chengsong},
    title = {{The Strength of Random Search on Automated Program Repair}},
    booktitle = {Proceedings of the 36th International Conference on Software Engineering},
    year = {2014},
    isbn = {978-1-4503-2756-5},
    pages = {254--265},
    doi = {10.1145/2568225.2568254},
    acmid = {2568254},
    publisher = {ACM},
} 

@inproceedings{Weimer2013AE,
    author = {Weimer, Westley and Fry, Zachary P. and Forrest, Stephanie},
    title = {{Leveraging Program Equivalence for Adaptive Program Repair: Models and First Results}},
    booktitle = {Proceedings of the 28th IEEE/ACM International Conference on Automated Software Engineering (ASE'13)},
    year = {2013},
    isbn = {978-1-4799-0215-6},
    location = {Silicon Valley, CA, USA},
    pages = {356--366},
    doi = {10.1109/ASE.2013.6693094},
    acmid = {3107702},
    publisher = {IEEE Press},
}

%Repair tools end

%Benchmarks of bugs papers beginning

@inproceedings{Hutchins1994Siemens,
    author = {Hutchins, Monica and Foster, Herb and Goradia, Tarak and Ostrand, Thomas},
    title = {{Experiments of the Effectiveness of Dataflow- and Controlflow-Based Test Adequacy Criteria}},
    booktitle = {Proceedings of the 16th International Conference on Software Engineering (ICSE '94)},
    year = {1994},
    isbn = {0-8186-5855-X},
    location = {Sorrento, Italy},
    pages = {191--200},
    numpages = {10},
    url = {http://dl.acm.org/citation.cfm?id=257734.257766},
    acmid = {257766},
    publisher = {IEEE Computer Society Press},
    address = {Los Alamitos, CA, USA},
} 

@article{Do2005SIR,
    author = {Do, Hyunsook and Elbaum, Sebastian and Rothermel, Gregg},
    title = {{Supporting Controlled Experimentation with Testing Techniques: An Infrastructure and its Potential Impact}},
    journal = {Empirical Software Engineering},
    issue_date = {October   2005},
    volume = {10},
    number = {4},
    month = oct,
    year = {2005},
    issn = {1382-3256},
    pages = {405--435},
    numpages = {31},
    url = {http://dx.doi.org/10.1007/s10664-005-3861-2},
    doi = {10.1007/s10664-005-3861-2},
    acmid = {1089928},
    publisher = {Kluwer Academic Publishers},
    address = {Hingham, MA, USA},
    keywords = {Software testing, controlled experimentation, experiment infrastructure, regression testing},
} 

@inproceedings{Lu2005BugBench,
    author = {Shan Lu and Zhenmin Li and Feng Qin and Lin Tan and Pin Zhou and Yuanyuan Zhou},
    title = {{BugBench: Benchmarks for Evaluating Bug Detection Tools}},
    booktitle = {Proceedings of the Workshop on the Evaluation of Software Defect Detection Tools},
    year = {2005},
}

@inproceedings{Dallmeier2007iBugs,
    author = {Dallmeier, Valentin and Zimmermann, Thomas},
    title = {{Extraction of Bug Localization Benchmarks from History}},
    booktitle = {Proceedings of the 22nd IEEE/ACM International Conference on Automated Software Engineering (ASE '07)},
    year = {2007},
    isbn = {978-1-59593-882-4},
    location = {Atlanta, Georgia, USA},
    pages = {433--436},
    numpages = {4},
    url = {http://doi.acm.org/10.1145/1321631.1321702},
    doi = {10.1145/1321631.1321702},
    acmid = {1321702},
    publisher = {ACM},
    address = {New York, NY, USA},
    keywords = {benchmarking, defect localization},
} 

@inproceedings{Just2014Defects4J,
    author = {Just, Ren{\'e} and Jalali, Darioush and Ernst, Michael D.},
    title = {{Defects4J: A Database of Existing Faults to Enable Controlled Testing Studies for Java Programs}},
    booktitle = {Proceedings of the 23rd International Symposium on Software Testing and Analysis},
    year = {2014},
    isbn = {978-1-4503-2645-2},
    pages = {437--440},
    doi = {10.1145/2610384.2628055},
    acmid = {2628055},
    publisher = {ACM},
}

@article{LeGoues2015ManyBugsIntroClass,
    author = {Claire {Le Goues} and Neal Holtschulte and Edward K. Smith and Yuriy Brun and Premkumar Devanbu and Stephanie Forrest and Westley Weimer},
    title = {{The ManyBugs and IntroClass Benchmarks for Automated Repair of C Programs}},
    journal = {IEEE Transactions on Software Engineering},
    issue_date = {December 2015},
    volume = {41},
    number = {12},
    month = dec,
    year = {2015},
    pages = {1236--1256},
    numpages = {21},
    publisher = {IEEE Press},
    address = {Piscataway, NJ, USA},
}

@techreport{Durieux2016IntroClassJava,
    author = {Thomas Durieux and Martin Monperrus},
    title = {{IntroClassJava: A Benchmark of 297 Small and Buggy Java Programs}},
    number = {\#hal-01272126},
    institution = {University of Lille},
    address = {University of Lille},
    year = {2016},
}

@inproceedings{Tan2017Codeflaws,
    author = {Tan, Shin Hwei and Yi, Jooyong and Yulis and Mechtaev, Sergey and Roychoudhury, Abhik},
    title = {{Codeflaws: A Programming Competition Benchmark for Evaluating Automated Program Repair Tools}},
    booktitle = {Proceedings of the 39th International Conference on Software Engineering Companion (ICSE-C '17)},
    year = {2017},
    isbn = {978-1-5386-1589-8},
    location = {Buenos Aires, Argentina},
    pages = {180--182},
    numpages = {3},
    url = {https://doi.org/10.1109/ICSE-C.2017.76},
    doi = {10.1109/ICSE-C.2017.76},
    acmid = {3098405},
    publisher = {IEEE Press},
    address = {Piscataway, NJ, USA},
    keywords = {automated program repair, benchmark, defect classes, empirical evaluation},
}

@inproceedings{Lin2017QuixBugs,
    author = {Lin, Derrick and Koppel, James and Chen, Angela and Solar-Lezama, Armando},
    title = {{QuixBugs: A Multi-Lingual Program Repair Benchmark Set Based on the Quixey Challenge}},
    booktitle = {ACM SIGPLAN International Conference on Systems, Programming, Languages, and Applications: Software for Humanity},
    year = {2017},
    isbn = {978-1-4503-5514-8},
    location = {Vancouver, BC, Canada},
    pages = {55--56},
    doi = {10.1145/3135932.3135941},
    acmid = {3135941},
    publisher = {ACM},
} 

@inproceedings{Saha2018BugsDotjar,
    author = {Saha, Ripon K. and Lyu, Yingjun and Lam, Wing and Yoshida, Hiroaki and Prasad, Mukul R.},
    title = {{Bugs.jar: A Large-scale, Diverse Dataset of Real-world Java Bugs}},
    booktitle = {International Conference on Mining Software Repositories},
    year = {2018},
    isbn = {978-1-4503-5716-6},
    pages = {10--13},
    doi = {10.1145/3196398.3196473},
    acmid = {3196473},
    publisher = {ACM},
}

@inproceedings{Madeiral2019Bears,
    author = {Fernanda Madeiral and Simon Urli and Marcelo Maia and Martin Monperrus},
    title = {{Bears: An Extensible Java Bug Benchmark for Automatic Program Repair Studies}},
    booktitle = {Proceedings of the 26th IEEE International Conference on Software Analysis, Evolution and Reengineering (SANER '19)},
    year = {2019},
    pages = {468--478},
    publisher = {IEEE},
    address = {Hangzhou, China},
}

@misc{Azevedo2018DroidBugs,
    author = {Larissa Azevedo and Altino Dantas and Celso G. Camilo-Junior},
    title = {{DroidBugs: An Android Benchmark for Automated Program Repair}},
    year = {2018},
    eprint = {1809.07353},
    archivePrefix = {arXiv},
    primaryClass = {cs.SE}
}

@inproceedings{Gyimesi2019BugsJS,
    author = {Gyimesi, P\'eter and Vancsics, B\'ela and Stocco, Andrea and Mazinanian, Davood and Besz\'edes, \'Arp\'ad and Ferenc, Rudolf and Mesbah, Ali},
    title = {{BugsJS: A Benchmark of JavaScript Bugs}},
    booktitle = {{Proceedings of the 12th International Conference on Software Testing, Verification, and Validation (ICST '19)}},
    year = {2019},
    location = {Xian, China},
    pages = {1--12},
    publisher = {IEEE Computer Society},
    address = {Washington, DC, USA},
}

%Benchmarks of bugs papers end

%Evaluations beginning

@article{Martinez2017experiment,
    author = {Martinez, Matias and Durieux, Thomas and Sommerard, Romain and Xuan, Jifeng and Monperrus, Martin},
    title = {{Automatic Repair of Real Bugs in Java: A Large-scale Experiment on the Defects4J Dataset}},
    journal = {Empirical Software Engineering},
    issue_date = {August    2017},
    volume = {22},
    number = {4},
    year = {2017},
    issn = {1382-3256},
    pages = {1936--1964},
    doi = {10.1007/s10664-016-9470-4},
    acmid = {3128829},
    publisher = {Kluwer Academic Publishers},
} 

@article{Motwani2018evaluation,
    author = {Motwani, Manish and Sankaranarayanan, Sandhya and Just, Ren{\'e} and Brun, Yuriy},
    title = {{Do automated program repair techniques repair hard and important bugs?}},
    journal = {Empirical Software Engineering},
    volume = {23},
    number = {5},
    year = {2018},
    issn = {1573-7616},
    pages = {2901--2947},
    doi = {10.1007/s10664-017-9550-0},
    publisher = {Springer US},
}

@inproceedings{Ye2019StudyQuixBugs,
    author = {He Ye and Matias Martinez and Thomas Durieux and Martin Monperrus},
    title = {{A Comprehensive Study of Automatic Program Repair on the QuixBugs Benchmark}},
    booktitle = {International Workshop on Intelligent Bug Fixing (co-located with SANER)},
    year = {2019},
    pages = {1--10},
    publisher = {IEEE},
}
@incollection{zhang2019support,
  title={Support vector machine},
  author={Zhang, Dengsheng},
  booktitle={Fundamentals of Image Data Mining},
  pages={179--205},
  year={2019},
  publisher={Springer}
}

@inproceedings{Boser1992SVM,
author = {Boser, Bernhard E. and Guyon, Isabelle M. and Vapnik, Vladimir N.},
title = {A Training Algorithm for Optimal Margin Classifiers},
year = {1992},
isbn = {089791497X},
publisher = {Association for Computing Machinery},
address = {New York, NY, USA},
url = {https://doi.org/10.1145/130385.130401},
doi = {10.1145/130385.130401},
abstract = {A training algorithm that maximizes the margin between the training patterns and the decision boundary is presented. The technique is applicable to a wide variety of the classification functions, including Perceptrons, polynomials, and Radial Basis Functions. The effective number of parameters is adjusted automatically to match the complexity of the problem. The solution is expressed as a linear combination of supporting patterns. These are the subset of training patterns that are closest to the decision boundary. Bounds on the generalization performance based on the leave-one-out method and the VC-dimension are given. Experimental results on optical character recognition problems demonstrate the good generalization obtained when compared with other learning algorithms.},
booktitle = {Proceedings of the Fifth Annual Workshop on Computational Learning Theory},
pages = {144–152},
numpages = {9},
location = {Pittsburgh, Pennsylvania, USA},
series = {COLT '92}
}

@inproceedings{Tong2001SVMA,
author = {Tong, Simon and Chang, Edward},
title = {Support Vector Machine Active Learning for Image Retrieval},
year = {2001},
isbn = {1581133944},
publisher = {Association for Computing Machinery},
address = {New York, NY, USA},
url = {https://doi.org/10.1145/500141.500159},
doi = {10.1145/500141.500159},
abstract = {Relevance feedback is often a critical component when designing image databases. With these databases it is difficult to specify queries directly and explicitly. Relevance feedback interactively determinines a user's desired output or query concept by asking the user whether certain proposed images are relevant or not. For a relevance feedback algorithm to be effective, it must grasp a user's query concept accurately and quickly, while also only asking the user to label a small number of images. We propose the use of a support vector machine active learning algorithm for conducting effective relevance feedback for image retrieval. The algorithm selects the most informative images to query a user and quickly learns a boundary that separates the images that satisfy the user's query concept from the rest of the dataset. Experimental results show that our algorithm achieves significantly higher search accuracy than traditional query refinement schemes after just three to four rounds of relevance feedback.},
booktitle = {Proceedings of the Ninth ACM International Conference on Multimedia},
pages = {107–118},
numpages = {12},
keywords = {image retrieval, relevance feedback, query concept, support vector machines, active learning},
location = {Ottawa, Canada},
series = {MULTIMEDIA '01}
}

@INPROCEEDINGS{Ho1995RandomForest,
  author={ {Tin Kam Ho}},
  booktitle={Proceedings of 3rd International Conference on Document Analysis and Recognition}, 
  title={Random decision forests}, 
  year={1995},
  volume={1},
  number={},
  pages={278-282 vol.1},
  doi={10.1109/ICDAR.1995.598994}}

@article{HORNIK1989359Multilayer,
title = {Multilayer feedforward networks are universal approximators},
journal = {Neural Networks},
volume = {2},
number = {5},
pages = {359-366},
year = {1989},
issn = {0893-6080},
doi = {https://doi.org/10.1016/0893-6080(89)90020-8},
url = {https://www.sciencedirect.com/science/article/pii/0893608089900208},
author = {Kurt Hornik and Maxwell Stinchcombe and Halbert White},
keywords = {Feedforward networks, Universal approximation, Mapping networks, Network representation capability, Stone-Weierstrass Theorem, Squashing functions, Sigma-Pi networks, Back-propagation networks},
abstract = {This paper rigorously establishes that standard multilayer feedforward networks with as few as one hidden layer using arbitrary squashing functions are capable of approximating any Borel measurable function from one finite dimensional space to another to any desired degree of accuracy, provided sufficiently many hidden units are available. In this sense, multilayer feedforward networks are a class of universal approximators.}
}
@book{Vapnik1995,
author = {Vapnik, Vladimir N.},
title = {The Nature of Statistical Learning Theory},
year = {1995},
isbn = {0387945598},
publisher = {Springer-Verlag},
address = {Berlin, Heidelberg}
}

@inproceedings{Smith2015,
    author = {Smith, Edward K. and Barr, Earl T. and Le Goues, Claire and Brun, Yuriy},
    title = {{Is the Cure Worse Than the Disease? Overfitting in Automated Program Repair}},
    booktitle = {Proceedings of the 10th Joint Meeting on Foundations of Software Engineering (ESEC/FSE '15)},
    year = {2015},
    isbn = {978-1-4503-3675-8},
    pages = {532--543},
    doi = {10.1145/2786805.2786825},
    acmid = {2786825},
    publisher = {ACM},
}

@inproceedings{Le2018overfitting,
    author = {Le, Xuan-Bach D. and Thung, Ferdian and Lo, David and Goues, Claire Le},
    title = {{Overfitting in semantics-based automated program repair}},
    booktitle = {Proceedings of the 40th International Conference on Software Engineering (ICSE '18)},
    year = {2018},
    isbn = {978-1-4503-5638-1},
    location = {Gothenburg, Sweden},
    pages = {163--163},
    numpages = {1},
    url = {http://doi.acm.org/10.1145/3180155.3182536},
    doi = {10.1145/3180155.3182536},
    acmid = {3182536},
    publisher = {ACM},
    address = {New York, NY, USA},
    keywords = {automated program repair, patch overfitting, program synthesis, symbolic execution},
} 

%Evaluations end

@inproceedings{Martinez2014,
    author = {Martinez, Matias and Weimer, Westley and Monperrus, Martin},
    title = {{Do the Fix Ingredients Already Exist? An Empirical Inquiry into the Redundancy Assumptions of Program Repair Approaches}},
    booktitle = {Proceedings of the 36th International Conference on Software Engineering (ICSE Companion 2014)},
    year = {2014},
    isbn = {978-1-4503-2768-8},
    location = {Hyderabad, India},
    pages = {492--495},
    numpages = {4},
    url = {http://doi.acm.org/10.1145/2591062.2591114},
    doi = {10.1145/2591062.2591114},
    acmid = {2591114},
    publisher = {ACM},
    address = {New York, NY, USA},
    keywords = {automatic software repair, mining software repositories},
}

@misc{codeforces,
	author = {Codeforces},
	title = {Codeforces. Programming competitions and contests, programming community.},
	howpublished = {\url{https://codeforces.com/}},
	year = {2018},
}

@incollection{grid5000,
    author = {Balouek, Daniel and Carpen Amarie, Alexandra and Charrier, Ghislain and Desprez, Fr{\'e}d{\'e}ric and Jeannot, Emmanuel and Jeanvoine, Emmanuel and L{\`e}bre, Adrien and Margery, David and Niclausse, Nicolas and Nussbaum, Lucas and Richard, Olivier and P{\'e}rez, Christian and Quesnel, Flavien and Rohr, Cyril and Sarzyniec, Luc},
    title = {{Adding Virtualization Capabilities to the Grid'5000 Testbed}},
    booktitle = {Cloud Computing and Services Science},
    editor = {Ivanov, Ivan I. and van Sinderen, Marten and Leymann, Frank and Shan, Tony},
    series = {Communications in Computer and Information Science},
    volume = {367},
    pages = {3--20},
    isbn = {978-3-319-04518-4},
    doi = {10.1007/978-3-319-04519-1\_1},
    year = {2013},
    publisher = {Springer International Publishing},
    address = {Cham},
}

@inproceedings{Sobreira2018defects4jdissection,
    author = {Victor Sobreira and Thomas Durieux and Fernanda Madeiral and Martin Monperrus and Marcelo A. Maia},
    title = {{Dissection of a Bug Dataset: Anatomy of 395 Patches from Defects4J}},
    booktitle = {Proceedings of the 25th IEEE International Conference on Software Analysis, Evolution and Reengineering (SANER '18)},
    year = {2018},
    isbn = {978-1-5386-4970-1},
    pages = {130--140},
    doi = {10.1109/SANER.2018.8330203},
    publisher = {IEEE},
    address = {Campobasso, Italy},
}
@article{rice1976algorithm,
  title={The algorithm selection problem},
  author={Rice, John R. and others},
  journal={Advances in computers},
  volume={15},
  number={65-118},
  pages={5},
  year={1976}
}
@inproceedings{oliveira2019footprints,
  title={Footprints of fitness functions in search-based software testing},
  author={Oliveira, Carlos and Aleti, Aldeida and Li, Yuan-Fang and Abdelrazek, Mohamed},
  booktitle={Proceedings of the Genetic and Evolutionary Computation Conference},
  pages={1399--1407},
  year={2019}
}
@article{Yu2019,
    author = {Yu, Zhongxing and Martinez, Matias and Danglot, Benjamin and Durieux, Thomas and Monperrus, Martin},
    title = {{Alleviating Patch Overfitting with Automatic Test Generation: A Study of Feasibility and Effectiveness for the Nopol Repair System}},
    journal = {Empirical Software Engineering},
    issue_date = {February  2019},
    volume = {24},
    number = {1},
    month = feb,
    year = {2019},
    issn = {1382-3256},
    pages = {33--67},
    numpages = {35},
    url = {https://doi.org/10.1007/s10664-018-9619-4},
    doi = {10.1007/s10664-018-9619-4},
    acmid = {3315702},
    publisher = {Kluwer Academic Publishers},
    address = {Norwell, MA, USA},
    keywords = {Automatic test case generation, Patch overfitting, Program repair, Synthesis-based repair},
}
@article{munoz2018instance,
  title={Instance spaces for machine learning classification},
  author={Mu{\~n}oz, Mario A and Villanova, Laura and Baatar, Davaatseren and Smith-Miles, Kate},
  journal={Machine Learning},
  volume={107},
  number={1},
  pages={109--147},
  year={2018},
  publisher={Springer}
}

@techreport{Ye2019ODS,
Author = {He Ye and Jian Gu and Matias Martinez and Thomas Durieux and Martin Monperrus},
Title = {Automated Classification of Overfitting Patches with Statically Extracted Code Features},
Year = {2019},
Eprint = {arXiv:1910.12057},
url = {http://arxiv.org/pdf/1910.12057},
number = {1910.12057},
institution = {arXiv}
}

@techreport{Yu2019XCRF,
Author = {Zhongxing Yu and Matias Martinez and Tegawendé F. Bissyandé and Martin Monperrus},
Title = {Learning the Relation between Code Features and Code Transforms with Structured Prediction},
Year = {2019},
Eprint = {arXiv:1907.09282},
url = {http://arxiv.org/pdf/1907.09282},
number = {1907.09282},
institution = {arXiv}
}

@article{wei2015variable,
  title={Variable importance analysis: a comprehensive review},
  author={Wei, Pengfei and Lu, Zhenzhou and Song, Jingwen},
  journal={Reliability Engineering \& System Safety},
  volume={142},
  pages={399--432},
  year={2015},
  publisher={Elsevier}
}

@article{martinez2017automatic,
  title={Automatic repair of real bugs in java: A large-scale experiment on the defects4j dataset},
  author={Martinez, Matias and Durieux, Thomas and Sommerard, Romain and Xuan, Jifeng and Monperrus, Martin},
  journal={Empirical Software Engineering},
  volume={22},
  number={4},
  pages={1936--1964},
  year={2017},
  publisher={Springer}
}

@ARTICLE{ckjm,
author={D. {Spinellis}},
journal={IEEE Software},
title={Tool writing: a forgotten art? (software tools)},
year={2005},
volume={22},
number={4},
pages={9-11},
doi={10.1109/MS.2005.111},
ISSN={},
month={July},}

@book{stats_learning,
    title = {The Elements of Statistical Learning - Data Mining, Inference and Prediction},
    author = {T. Hastie, R. Tibshirani and J. Friedman},
    year = {2009},
    isbn = {9780387848570},
    Publisher = {Springer-Verlag New York}
}

@inproceedings{ckjm_defects,
author = {Jureczko, Marian and Spinellis, Diomidis},
year = {2010},
month = {06},
pages = {},
title = {Using Object-Oriented Design Metrics to Predict Software Defects},
journal = {Models and Methods of System Dependability}
}

@INPROCEEDINGS{jct,
author={M. {Lumpe} and S. {Mahmud} and O. {Goloshchapova}},
booktitle={2011 26th IEEE/ACM International Conference on Automated Software Engineering (ASE 2011)},
title={jCT: A Java Code Tomograph},
year={2011},
volume={},
number={},
pages={616-619},
keywords={data mining;Java;program diagnostics;software metrics;Java code tomograph;software analysis;empirical software engineering;metrics data mining;metrics extraction;curated repositories;Qualitas Corpus;Helix;Java;Software systems;Data mining;Software measurement;Software engineering;Software metrics;Data mining;Reasoning about programs},
doi={10.1109/ASE.2011.6100139},
ISSN={},
month={Nov},}

@INPROCEEDINGS{jct_comparitive,
author={O. {Goloshchapova} and M. {Lumpe}},
booktitle={2013 22nd Australian Software Engineering Conference},
title={On the Application of Inequality Indices in Comparative Software Analysis},
year={2013},
volume={},
number={},
pages={117-126},
keywords={socio-economic effects;software metrics;statistical analysis;comparative software analysis;socio-economic inequality indices;Gini coefficient;Theil index;central tendency statistics;software metrics data;metrics distribution;ecological fallacies;macrolevel inference;microlevel analysis;organizational health;Indexes;Sociology;Statistics;Software metrics;Software systems;empirical software analysis;software metrics;inequality analysis;software evolution;measurement approaches},
}

@article{britton2013reversible,
  title={britton2013reversible},
  author={Britton, Tom and Jeng, Lisa and Carver, Graham and Cheak, Paul and Katzenellenbogen, Tomer},
  journal={Judge Bus. School, Univ. Cambridge, Cambridge, UK, Tech. Rep},
  year={2013}
}

@ARTICLE{testsuitegen, 
author={C. {Oliveira} and A. {Aleti} and L. {Grunske} and K. {Smith-Miles}}, 
journal={IEEE Transactions on Reliability}, 
title={Mapping the Effectiveness of Automated Test Suite Generation Techniques}, 
year={2018}, 
volume={67}, 
number={3}, 
pages={771-785}, 
}

@article{deeprepair,
  author    = {Martin White and
               Michele Tufano and
               Matias Martinez and
               Martin Monperrus and
               Denys Poshyvanyk},
  title     = {Sorting and Transforming Program Repair Ingredients via Deep Learning
               Code Similarities},
  journal   = {CoRR},
  volume    = {abs/1707.04742},
  year      = {2017},
  url       = {http://arxiv.org/abs/1707.04742},
  archivePrefix = {arXiv},
  eprint    = {1707.04742},
  timestamp = {Mon, 13 Aug 2018 16:47:09 +0200},
  biburl    = {https://dblp.org/rec/bib/journals/corr/WhiteTMMP17},
  bibsource = {dblp computer science bibliography, https://dblp.org}
}

@article{explainableAI,
  author    = {Wojciech Samek and  Thomas Wiegand and Klaus{-}Robert M{\"{u}}ller},
  title     = {Explainable Artificial Intelligence: Understanding, Visualizing and
               Interpreting Deep Learning Models},
  journal   = {CoRR},
  volume    = {abs/1708.08296},
  year      = {2017},
}

@Inbook{ckjmextended,
 author = {Jureczko, Marian and Spinellis, Diomidis},
 title = {Using Object-Oriented Design Metrics to Predict Software Defects},
 volume = {Models and Methodology of System Dependability},
 series = {Monographs of System Dependability},
 year = {2010},
 isbn = {978-83-7493-526-5},
 pages = {69-81},
 publisher = {Oficyna Wydawnicza Politechniki Wroclawskiej},
 address = {Wroclaw, Poland}
}

@article{featureimportance,
  title={Variable importance analysis: a comprehensive review},
  author={Wei, Pengfei and Lu, Zhenzhou and Song, Jingwen},
  journal={Reliability Engineering \& System Safety},
  volume={142},
  pages={399--432},
  year={2015},
  publisher={Elsevier}
}

@article{repairnator2019,
author = {Monperrus, Martin and Urli, Simon and Durieux, Thomas and Martinez, Matias and Baudry, Benoit and Seinturier, Lionel},
title = {Repairnator Patches Programs Automatically},
year = {2019},
issue_date = {July 2019},
publisher = {ACM},
volume = {2019},
doi = {10.1145/3349589},
journal = {Ubiquity},
}

@inproceedings{anti-pattern,
 author = {Tan, Shin Hwei and Yoshida, Hiroaki and Prasad, Mukul R. and Roychoudhury, Abhik},
 title = {Anti-patterns in Search-based Program Repair},
 booktitle = {ACM SIGSOFT International Symposium on Foundations of Software Engineering},
 year = {2016},
 isbn = {978-1-4503-4218-6},
 pages = {727--738},
}
@inproceedings{patchsim,
  title={Identifying patch correctness in test-based program repair},
  author={Xiong, Yingfei and Liu, Xinyuan and Zeng, Muhan and Zhang, Lu and Huang, Gang},
  booktitle={International Conference on Software Engineering},
  pages={789--799},
  year={2018},
  organization={ACM}
}

@INPROCEEDINGS{lee2015fixingdelegated,
author={X. D. {Le} and T. B. {Le} and D. {Lo}},
booktitle={2015 IEEE 26th International Symposium on Software Reliability Engineering (ISSRE)},
title={Should fixing these failures be delegated to automated program repair?},
year={2015},
volume={},
number={},
pages={427-437},
keywords={genetic algorithms;program debugging;search problems;software maintenance;software maintenance components;software production cost;software maintenance cost reduction;automatic software defect fixing;oracle;bug fixing process;genetic-programming-based automated program repair approaches;syntactically mutated programs;machine learning;genetic programming search;GenProg;precision value;recall value;F-measure value;AUC value;Maintenance engineering;Feature extraction;Computer bugs;Sociology;Statistics;Predictive models;Genetic programming;Automated Program Repair;Effectiveness Prediction;Effective Feature Design;Classification Techniques},
doi={10.1109/ISSRE.2015.7381836},
ISSN={null},
month={Nov},}

@inproceedings{Martinez2019Coming,
author = {Martinez, Matias and Monperrus, Martin},
title = {Coming: A Tool for Mining Change Pattern Instances from Git Commits},
year = {2019},
publisher = {IEEE Press},
url = {https://doi.org/10.1109/ICSE-Companion.2019.00043},
doi = {10.1109/ICSE-Companion.2019.00043},
booktitle = {Proceedings of the 41st International Conference on Software Engineering: Companion Proceedings},
pages = {79–82},
numpages = {4},
location = {Montreal, Quebec, Canada},
series = {ICSE ’19}
}
  
@inproceedings{Long2016Space,
author = {Long, Fan and Rinard, Martin},
title = {An Analysis of the Search Spaces for Generate and Validate Patch Generation Systems},
year = {2016},
isbn = {9781450339001},
publisher = {Association for Computing Machinery},
address = {New York, NY, USA},
url = {https://doi.org/10.1145/2884781.2884872},
doi = {10.1145/2884781.2884872},
booktitle = {Proceedings of the 38th International Conference on Software Engineering},
pages = {702–713},
numpages = {12},
keywords = {patch generation, search space, program repair},
location = {Austin, Texas},
series = {ICSE ’16}
}

@INPROCEEDINGS{Campos2012GZoltar,
  author={J. {Campos} and A. {Riboira} and A. {Perez} and R. {Abreu}},
  booktitle={2012 Proceedings of the 27th IEEE/ACM International Conference on Automated Software Engineering}, 
  title={GZoltar: an eclipse plug-in for testing and debugging}, 
  year={2012},
  volume={},
  number={},
  pages={378-381},}

@INPROCEEDINGS{Abreu2017Accuracy,
  author={R. {Abreu} and P. {Zoeteweij} and A. J. C. {van Gemund}},
  booktitle={Testing: Academic and Industrial Conference Practice and Research Techniques - MUTATION (TAICPART-MUTATION 2007)}, 
  title={On the Accuracy of Spectrum-based Fault Localization}, 
  year={2007},
  volume={},
  number={},
  pages={89-98},}
  
@inproceedings{Xiong2018Identifiying,
author = {Xiong, Yingfei and Liu, Xinyuan and Zeng, Muhan and Zhang, Lu and Huang, Gang},
title = {Identifying Patch Correctness in Test-Based Program Repair},
year = {2018},
isbn = {9781450356381},
publisher = {Association for Computing Machinery},
address = {New York, NY, USA},
url = {https://doi.org/10.1145/3180155.3180182},
doi = {10.1145/3180155.3180182},
booktitle = {Proceedings of the 40th International Conference on Software Engineering},
pages = {789–799},
numpages = {11},
location = {Gothenburg, Sweden},
series = {ICSE ’18}
}
  
@inproceedings{issta17-difftgen,
author = {Qi Xin  and  Steven  Reiss},
title = {Identifying Test-Suite-Overfitted Patches through Test Case Generation},
year = {2017},
isbn = {9781450350761},
publisher = {Association for Computing Machinery},
address = {New York, NY, USA},
url = {https://doi.org/10.1145/3092703.3092718},
doi = {10.1145/3092703.3092718},
booktitle = {Proceedings of the 26th ACM SIGSOFT International Symposium on Software Testing and Analysis},
pages = {226–236},
numpages = {11},
location = {Santa Barbara, CA, USA},
series = {ISSTA 2017}
}
 
@inproceedings{Le2019Reliability,
author = {Le, Xuan-Bach D. and Bao, Lingfeng and Lo, David and Xia, Xin and Li, Shanping and Pasareanu, Corina},
title = {On Reliability of Patch Correctness Assessment},
year = {2019},
publisher = {IEEE Press},
url = {https://doi.org/10.1109/ICSE.2019.00064},
doi = {10.1109/ICSE.2019.00064},
booktitle = {Proceedings of the 41st International Conference on Software Engineering},
pages = {524–535},
numpages = {12},
location = {Montreal, Quebec, Canada},
series = {ICSE ’19}
}
  
@INPROCEEDINGS{Yokoyama2017Evaluating,
  author={H. {Yokoyama} and Y. {Higo} and S. {Kusumoto}},
  booktitle={2017 8th International Workshop on Empirical Software Engineering in Practice (IWESEP)}, 
  title={Evaluating Automated Program Repair Using Characteristics of Defects}, 
  year={2017},
  volume={},
  number={},
  pages={47-52},}

@inproceedings{li2020DLfix,
author = {Li, Yi and Wang, Shaohua and Nguyen, Tien N.},
title = {DLFix: Context-Based Code Transformation Learning for Automated Program Repair},
year = {2020},
isbn = {9781450371216},
publisher = {Association for Computing Machinery},
address = {New York, NY, USA},
url = {https://doi.org/10.1145/3377811.3380345},
doi = {10.1145/3377811.3380345},
booktitle = {Proceedings of the ACM/IEEE 42nd International Conference on Software Engineering},
pages = {602–614},
numpages = {13},
keywords = {automated program repair, context-based code transformation learning, deep learning},
location = {Seoul, South Korea},
series = {ICSE '20}
}

@article{Liu2021Critical,
title = "A critical review on the evaluation of automated program repair systems",
journal = "Journal of Systems and Software",
volume = "171",
pages = "110817",
year = "2021",
issn = "0164-1212",
doi = "https://doi.org/10.1016/j.jss.2020.110817",
url = "http://www.sciencedirect.com/science/article/pii/S0164121220302156",
author = "Kui Liu and Li Li and Anil Koyuncu and Dongsun Kim and Zhe Liu and Jacques Klein and Tegawendé F. Bissyandé",
keywords = "Automated program repair, Evaluation, Assessment, Metrics",
}

@inproceedings{tian2020evaluating, 
  title={Evaluating Representation Learning of Code Changes for Predicting Patch Correctness in Program Repair}, 
  author={Tian, Haoye and Liu, Kui and Kabor{\'e}, Abdoul Kader and Koyuncu, Anil and Li, Li and Klein, Jacques and Bissyand{\'e}, Tegawend{\'e} F.},
  booktitle={Proceedings of the 35th IEEE/ACM International Conference on Automated Software Engineering}, 
  year={2020}, 
  publisher={ACM}
} 
@inproceedings{Liu2020EficacyTestSuite,
author = {Liu, Kui and Wang, Shangwen and Koyuncu, Anil and Kim, Kisub and Bissyand\'{e}, Tegawend\'{e} F. and Kim, Dongsun and Wu, Peng and Klein, Jacques and Mao, Xiaoguang and Traon, Yves Le},
title = {On the Efficiency of Test Suite Based Program Repair: A Systematic Assessment of 16 Automated Repair Systems for Java Programs},
year = {2020},
isbn = {9781450371216},
publisher = {Association for Computing Machinery},
address = {New York, NY, USA},
url = {https://doi.org/10.1145/3377811.3380338},
doi = {10.1145/3377811.3380338},
booktitle = {Proceedings of the ACM/IEEE 42nd International Conference on Software Engineering},
pages = {615–627},
numpages = {13},
keywords = {program repair, empirical assessment, efficiency, patch generation},
location = {Seoul, South Korea},
series = {ICSE '20}
}

@ARTICLE{Liu2018,
  author={K. {Liu} and D. {Kim} and T. F. {Bissyande} and S. {Yoo} and Y. {Le Traon}},
  journal={IEEE Transactions on Software Engineering}, 
  title={Mining Fix Patterns for FindBugs Violations}, 
  year={2018},
  volume={},
  number={},
  pages={1-1},
  doi={10.1109/TSE.2018.2884955}}

@article{Koyuncu2020FixMiner,
	Abstract = {Patching is a common activity in software development. It is generally performed on a source code base to address bugs or add new functionalities. In this context, given the recurrence of bugs across projects, the associated similar patches can be leveraged to extract generic fix actions. While the literature includes various approaches leveraging similarity among patches to guide program repair, these approaches often do not yield fix patterns that are tractable and reusable as actionable input to APR systems. In this paper, we propose a systematic and automated approach to mining relevant and actionable fix patterns based on an iterative clustering strategy applied to atomic changes within patches. The goal of FixMiner is thus to infer separate and reusable fix patterns that can be leveraged in other patch generation systems. Our technique, FixMiner, leverages Rich Edit Script which is a specialized tree structure of the edit scripts that captures the AST-level context of the code changes. FixMiner uses different tree representations of Rich Edit Scripts for each round of clustering to identify similar changes. These are abstract syntax trees, edit actions trees, and code context trees. We have evaluated FixMiner on thousands of software patches collected from open source projects. Preliminary results show that we are able to mine accurate patterns, efficiently exploiting change information in Rich Edit Scripts. We further integrated the mined patterns to an automated program repair prototype, PARFixMiner, with which we are able to correctly fix 26 bugs of the Defects4J benchmark. Beyond this quantitative performance, we show that the mined fix patterns are sufficiently relevant to produce patches with a high probability of correctness: 81{\%} of PARFixMiner's generated plausible patches are correct.},
	Author = {Koyuncu, Anil and Liu, Kui and Bissyand{\'e}, Tegawend{\'e}F. and Kim, Dongsun and Klein, Jacques and Monperrus, Martin and Le Traon, Yves},
	Da = {2020/05/01},
	Date-Added = {2020-10-22 06:54:15 +0000},
	Date-Modified = {2020-10-22 06:54:15 +0000},
	Doi = {10.1007/s10664-019-09780-z},
	Id = {Koyuncu2020},
	Isbn = {1573-7616},
	Journal = {Empirical Software Engineering},
	Number = {3},
	Pages = {1980--2024},
	Title = {FixMiner: Mining relevant fix patterns for automated program repair},
	Ty = {JOUR},
	Url = {https://doi.org/10.1007/s10664-019-09780-z},
	Volume = {25},
	Year = {2020},
	Bdsk-Url-1 = {https://doi.org/10.1007/s10664-019-09780-z},
	Bdsk-Url-2 = {http://dx.doi.org/10.1007/s10664-019-09780-z}}

@inproceedings{Liu2019Tbar,
author = {Liu, Kui and Koyuncu, Anil and Kim, Dongsun and Bissyand\'{e}, Tegawend\'{e} F.},
title = {TBar: Revisiting Template-Based Automated Program Repair},
year = {2019},
isbn = {9781450362245},
publisher = {Association for Computing Machinery},
address = {New York, NY, USA},
url = {https://doi.org/10.1145/3293882.3330577},
doi = {10.1145/3293882.3330577},
abstract = {We revisit the performance of template-based APR to build comprehensive knowledge about the effectiveness of fix patterns, and to highlight the importance of complementary steps such as fault localization or donor code retrieval. To that end, we first investigate the literature to collect, summarize and label recurrently-used fix patterns. Based on the investigation, we build TBar, a straightforward APR tool that systematically attempts to apply these fix patterns to program bugs. We thoroughly evaluate TBar on the Defects4J benchmark. In particular, we assess the actual qualitative and quantitative diversity of fix patterns, as well as their effectiveness in yielding plausible or correct patches. Eventually, we find that, assuming a perfect fault localization, TBar correctly/plausibly fixes 74/101 bugs. Replicating a standard and practical pipeline of APR assessment, we demonstrate that TBar correctly fixes 43 bugs from Defects4J, an unprecedented performance in the literature (including all approaches, i.e., template-based, stochastic mutation-based or synthesis-based APR).},
booktitle = {Proceedings of the 28th ACM SIGSOFT International Symposium on Software Testing and Analysis},
pages = {31–42},
numpages = {12},
keywords = {fix pattern, empirical assessment, Automated program repair},
location = {Beijing, China},
series = {ISSTA 2019}
}
@inproceedings{liu2019avatar,
  Author = {Liu, Kui and Koyuncu, Anil and Kim, Dongsun and F. Bissyand{\'e}, Tegawend{\'e}},
  Title = {{AVATAR:} Fixing Semantic Bugs with Fix Patterns of Static Analysis Violations},
  Booktitle = {Proceedings of the 26th IEEE International Conference on Software Analysis, Evolution, and Reengineering},
  pages={456--467},
  year={2019},
  organization={IEEE}
}

@inproceedings{Lin2020Understanding,
author = {Lin, Bo and Wang, Shangwen and Wen, Ming and Zhang, Zhang and Wu, Hongjun and Qin, Yihao and Mao, Xiaoguang},
year = {2020},
month = {10},
pages = {},
title = {Understanding the Non-Repairability Factors of Automated Program Repair Techniques}
}

@INPROCEEDINGS{Liu2019FLbias,  author={K. {Liu} and A. {Koyuncu} and T. F. {Bissyandé} and D. {Kim} and J. {Klein} and Y. {Le Traon}},  booktitle={2019 12th IEEE Conference on Software Testing, Validation and Verification (ICST)},   title={You Cannot Fix What You Cannot Find! An Investigation of Fault Localization Bias in Benchmarking Automated Program Repair Systems},   year={2019},  volume={},  number={},  pages={102-113},  doi={10.1109/ICST.2019.00020}}

@MISC{appendix,
author = {Appendix},
title = {Appendix E-APR},
month = November,
year = {2020},
howpublished={\url{https://github.com/UPHF/eapr}}
}

@article{Wang2020AutomatedPC,
  title={Automated Patch Correctness Assessment: How Far are We?},
  author={Shangwen Wang and M. Wen and Bo Lin and Hongjun Wu and Yihao Qin and Deqing Zou and X. Mao and Hai Jin},
  journal={2020 35th IEEE/ACM International Conference on Automated Software Engineering (ASE)},
  year={2020},
  pages={968-980}
}

@techreport{Ginelli2020,
Author = {Davide Ginelli and Matias Martinez and
Leonardo Mariani and Martin Monperrus},
Title = {A Comprehensive Study of Code-removal Patches in Automated Program Repair},
Year = {2020},
Eprint = {arXiv:2012.06264},
url = {http://arxiv.org/pdf/2012.06264},
number = {2012.06264},
institution = {arXiv}
}
